# Supplementary material for: Convergence of Consensus-Based Particle Methods for Nonconvex Bi-Level Optimization
Source: arXiv:2605.19667 source file (2026-05-19)
Supplement: Supplementary file 1 [file appendix.tex]

\section{Global convergence proof}
\newcommand{\alphaGs}{\alpha_G^{(s)}}
\newcommand{\alphaLs}{\alpha_L^{(s)}}
\newcommand{\alphaGh}{\alpha_G^{(h)}}

We first consider the following min-min problem,

\begin{equation}
    \min_{\theta \in \Theta} G(\theta),
\qquad
\Theta := \arg\min_{\theta} L(\theta).
\end{equation}

We assume $|G(x)-G(y)|\le L_{G,M}\|x-y\|$ and $|L(x)-L(y)|\le L_{L,M}\|x-y\|$, for all $\|x\|,\|y\|\leq M$.

{\color{red}{furthermore, we assume the inverse continuity property holds for $G$ inside $\Theta$.}}

We define the soft-quantile $q_{\beta,\tau}^L[\rho]$ is the solution w.r.t $q(\rho)$ of the following function
\begin{equation}
\int s\!\left(\frac{q(\rho)-L(\theta)}{\tau}\right)\rho(d\theta)\;=\;\beta.
\end{equation}
where $s(u)\approx 1$ as $u\gg 0$, $s(u)\approx 0$ as $u\ll 0$ and $|s(u)-s(v)|\le L_s|u-v|$, $\forall u,v$.
%{\color{blue} make the assumptions on $s$ and $\beta$.}

{\color{red} How do we find $q$ with an algorithm?}

\begin{remark}
Here $s(\cdot)$ can be a sigmoid (softmax) function which continuously approximate a step function behavior. 
When $\tau\to 0$, $s(\cdot)$ behaves like a step function, the solution of $q$ is to find a $L(\theta)$ such that the integration becomes $\int_{L(\theta) \ge q} 0 \rho(d\theta) + \int_{L(\theta)\le q} 1 \rho(d\theta) =\beta$. 
In the general case of $\tau > 0$, 
the integration can be written as $\int_{L(\theta) \ge q} s^{(-)} \rho(d\theta) + \int_{L(\theta)\le q} s^{(+)}  \rho(d\theta) =\beta$
\end{remark}

\begin{remark}
$\frac{1}{\tau}$ can be understood as a temperature like hyperparameter controlling extent of this approximation. The relationship between $\alpha_L=\frac{1}{\tau}$ and $\alphaGs$ (see below) decides which softmax term dominates the other. The multiplication of two softmax can be visually thought of as amplitude modulation.
\end{remark}

%{\color{blue} give an example of such function: e.g., sigmoid}

For discrete sampling $\rho_k^N=\frac{1}{N}\sum_{i=1}^N\delta_{\theta_k^i}$, it becomes

\begin{equation}
\frac1N\sum_{i=1}^N s\!\left(\frac{q-L(\theta_k^i)}{\tau}\right)=\beta.    
\end{equation}

The soft-consensus point

\begin{equation}
 m_{\alphaGs,\beta,\tau}^{G,L}(\rho)=\frac{\int \theta e^{-\alphaGs G(\theta)}\,s\!\left(\frac{q_{\beta,\tau}^L[\rho]-L(\theta)}{\tau}\right)\rho(d\theta)}{\int e^{-\alphaGs G(\theta)}\,s\!\left(\frac{q_{\beta,\tau}^L[\rho]-L(\theta)}{\tau}\right)\rho(d\theta)}
\end{equation}

and its discrete version is
\begin{equation}
m_{\alphaGs,\beta,\tau}^{G,L}(\rho_k^N)
=
\frac{\sum_{i=1}^N \theta_k^i\,e^{-\alphaGs G(\theta_k^i)}\,\pi_k^i}
{\sum_{j=1}^N e^{-\alphaGs G(\theta_k^j)}\,\pi_k^j}.
\end{equation}

where 

\begin{equation}
\pi_{k}^i \;=\; s\!\left(\frac{q_{\beta,\tau}^L[\rho_k^N]-L(\theta_k^i)}{\tau}\right)\in[0,1].
\end{equation}

As $\tau\to 0^+$, it becomes the the  $\beta$-quantile of the set ${\{L(\theta_t^i)\}}_{i=1}^N$, i.e., 

\begin{equation}
    m_{\alphaGh,\beta}^{G,L}(\rho_k^N)
=
\frac{\sum\limits_{i:\,L(\theta_{k}^i)\le q_\beta^L[\rho_k^N]}
\theta_{k}^i\,e^{-\alphaGh G(\theta_{k}^i)}}{
\sum\limits_{j:\,L(\theta_k^j)\le q_\beta^L[\rho_k^N]}
e^{-\alphaGh G(\theta_k^j)}
},
\qquad
q_\beta^L[\rho_k^N]=L(\theta_k^{\#\lceil\beta N\rceil}).
\end{equation}

% \begin{assumption}
%     \begin{equation}
%         \|D(u)-D(v)\|\le L_D\|u-v\|,\qquad \forall u,v\in B_{2M}.
%     \end{equation}
% \end{assumption}

We propose the following Euler-Maruyama discrete particle update rule,

\begin{equation}
    \theta_{k+1,\tau}^i
=
\theta_{k,\tau}^i
-\Delta t\,\lambda\Bigl(\theta_{k,\tau}^i-m_{\alphaGs,\beta,\tau}^{G,L}(\rho_{k,\tau}^N)\Bigr)
+\sqrt{\Delta t}\,\sigma\,D\Bigl(\theta_{k,\tau}^i-m_{\alphaGs,\beta,\tau}^{G,L}(\rho_{k,\tau}^N)\Bigr)\,B_k^i,
\qquad i=1,\dots,N,
\end{equation}

where $B_k^i\sim\mathcal{N}(0,I_{d\times d})$ i.i.d., $\rho_{k,\tau}^N=\frac1N\sum_{i=1}^N\delta_{\theta_{k,\tau}^i}$.

We further define the continuous particle system $\Theta_{t,\tau}^{i,N}$ and mean-field limit $\bar\Theta_t$,

\begin{equation}
    d\Theta_{t,\tau}^{i,N}
=
-\lambda\Bigl(\Theta_{t,\tau}^{i,N} -  m_{\alphaGs,\beta,\tau}^{G,L}(\rho_t^N)\Bigr)\,dt
+
\sigma D\Bigl(\Theta_{t,\tau}^{i,N} - m_{\alphaGs,\beta,\tau}^{G,L}(\rho_t^N)\Bigr)\,dW_t^i,
\end{equation}

where $\rho_t^N := \frac1N \sum_{j=1}^N \delta_{\Theta_{t,\tau}^{j,N}},$

Now define the mean field dynamic

\begin{equation}
d\bar\Theta_{t,\tau}^i
=
-\lambda(\bar\Theta_{t,\tau}^i - m_{\alphaGs,\beta,\tau}^{G,L}(\rho_t))dt
+
\sigma D(\bar\Theta_{t,\tau}^i - m_{\alphaGs,\beta,\tau}^{G,L}(\rho_t)) dW_t^i
\end{equation}

where $\rho_t := \mathrm{Law}(\bar\Theta_t)$. The final output is 

\begin{equation}
    \widehat\theta_K^N := \frac1N\sum_{i=1}^N\theta_{k,\tau}^i,
\qquad
\underbrace{\widehat\Theta_T^N := \frac1N\sum_{i=1}^N\Theta_{t,\tau}^{i,N}}_{\text{continuous path particle dynamic}},
\qquad
\underbrace{\widehat{\bar\Theta}_T^N := \frac1N\sum_{i=1}^N\bar\Theta_{t,\tau}^i}_{\textbf{mean field particle dynamic}},
\qquad
\underbrace{\widehat{\bar\Theta}_{T,0}^N := \frac1N\sum_{i=1}^N\bar\Theta_{t,0}^i}_{\text{CB2O mean field particle dynamic}},
\end{equation}

Notice that,

\begin{equation}
    \|\widehat\theta_K^N-\theta^*\|_2^2
\le
4\|\widehat\theta_K^N-\widehat\Theta_T^N\|_2^2
+
4\|\widehat\Theta_T^N-\widehat{\bar\Theta}_T^N\|_2^2
+
4\|\widehat{\bar\Theta}_T^N-\widehat{\bar\Theta}_{T,0}^N\|_2^2
+
4\|\widehat{\bar\Theta}_{T,0}^N-\theta^\star\|_2^2.
\end{equation}

{\color{red} Let $\Omega_M$ denote the sigma algebra of the configration space corresponding to $B_{0,M}$ (ball with radius $M$ center at origin) where the lower level objective is global Liptischtz, i.e.
$\Omega_M=\{B_{0,M}, \emptyset, B^c_{0,M}\}$ where we use $B^c_{0,M}$ to denote the complement of the ball $B_{0,M}$.} 
By taking the expectation over $\Omega_M$,
%{\color{blue} give the definition.}

\begin{equation}\label{eq:terms}
    \frac{1}{4}\mathbb{E}\bigl[\|\widehat\theta_K^N-\theta^*\|_2^2 \mid \Omega_M\bigr]
\le
\mathbb{E}\bigl[\|\widehat\theta_K^N-\widehat\Theta_T^N\|_2^2 \mid \Omega_M\bigr]
+
\mathbb{E}\bigl[\|\widehat\Theta_T^N-\widehat{\bar\Theta}_T^N\|_2^2 \mid \Omega_M\bigr]
+
\mathbb{E}\bigl[\|\widehat{\bar\Theta}_T^N-\widehat{\bar\Theta}_{T,0}^N\|_2^2 \mid \Omega_M\bigr]
+
\mathbb{E}\bigl[\|\widehat{\bar\Theta}_{T,0}^N-\theta^\star]\|_2^2 \mid \Omega_M\bigr]
\end{equation}
Below, we bound each of the terms on the right-hand side of the above inequity. 

\textbf{The first term of \eqref{eq:terms}:}

\begin{equation}
  \underbrace{\|\widehat\theta_K^N-\widehat\Theta_T^N\|_2^2}_{\text{continuous path particle dynamic}}
=
\left\|\frac1N\sum_{i=1}^N(\theta_{k,\tau}^i-\Theta_{t,\tau}^{i,N})\right\|_2^2
\le
\frac1N\sum_{i=1}^N\|\theta_{k,\tau}^i-\Theta_{t,\tau}^{i,N}\|_2^2.
\end{equation}

By taking the expectation over $\Omega_M$ and notice $\mathbb{P}(\Omega_M)\ge 1-\delta\ge 1/2$,

\begin{equation}
    \mathbb{E}\left[\frac1N\sum_{i=1}^N\|\theta_{k,\tau}^i-\Theta_{t,\tau}^{i,N}\|_2^2 \mid \Omega_M\right]
=
\frac{\mathbb{E}\left[\frac1N\sum_{i=1}^N\|\theta_{k,\tau}^i-\Theta_{t,\tau}^{i,N}\|_2^2\,\mathbf{1}_{\Omega_M}\right]}{\mathbb{P}(\Omega_M)}
\le
2\,\mathbb{E}\left[\frac1N\sum_{i=1}^N\|\theta_{k,\tau}^i-\Theta_{t,\tau}^{i,N}\|_2^2\right].
\end{equation}

By applying classical convergence results for numerical schemes for SDEs \cite{platen1999introduction},

\begin{equation}
    \mathbb{E}\left[\frac1N\sum_{i=1}^N\|\theta_{k,\tau}^i-\Theta_{t,\tau}^{i,N}\|_2^2\right]
\le
C_{\mathrm{NA}}(\Delta t)^{2m}.
\end{equation}

\textbf{For the second term of \eqref{eq:terms}:} 
$$
\underbrace{\mathbb{E}\bigl[\|\widehat\Theta_T^N-\widehat{\bar\Theta}_T^N\|_2^2 \mid \Omega_M\bigr]}_{\text{Continuous path particle v.s.~mean field particle}},
$$
we denotes

\begin{equation}
    b(x,\rho)=-\lambda\bigl(x-m_{\alpha,\beta,\tau}^{G,L}(\rho)\bigr),\qquad
a(x,\rho)=\sigma\,D\bigl(x-m_{\alpha,\beta,\tau}^{G,L}(\rho)\bigr).
\end{equation}

In consequence,

\begin{align}
    d\Theta_{t,\tau}^{i,N}
&=
b\!\left(\Theta_{t,\tau}^{i,N},\,\rho_t^N\right)\,dt
+
a\!\left(\Theta_{t,\tau}^{i,N},\,\rho_t^N\right)\,dW_t^i,\\
d\bar\Theta_{t,\tau}^i
&=
b\!\left(\bar\Theta_{t,\tau}^i,\,\rho_t\right)\,dt
+
a\!\left(\bar\Theta_{t,\tau}^i,\,\rho_t\right)\,dW_t^i.
\end{align}

We define the error $e_t^i:=\Theta_{t,\tau}^{i,N}-\bar\Theta_{t,\tau}^i$, thus,

\begin{align}
    \begin{aligned}
de_t^i=
\Bigl(b(\Theta_{t,\tau}^{i,N},\rho_t^N)-b(\bar\Theta_{t,\tau}^i,\rho_t)\Bigr)\,dt
+
\Bigl(a(\Theta_{t,\tau}^{i,N},\rho_t^N)-a(\bar\Theta_{t,\tau}^i,\rho_t)\Bigr)\,dW_t^i.
\end{aligned}
\end{align}

By applying Ito's Lemma,

\begin{equation}
    \begin{aligned}
d\|e_t^i\|^2
&=2\langle e_t^i,\,de_t^i\rangle+\|a(\Theta_{t,\tau}^{i,N},\rho_t^N)-a(\bar\Theta_{t,\tau}^i,\rho_t)\|^2\,dt\\
&=2\Bigl\langle e_t^i,\,b(\Theta_{t,\tau}^{i,N},\rho_t^N)-b(\bar\Theta_{t,\tau}^i,\rho_t)\Bigr\rangle dt\\
&\quad +2\Bigl\langle e_t^i,\,\bigl(a(\Theta_{t,\tau}^{i,N},\rho_t^N)-a(\bar\Theta_{t,\tau}^i,\rho_t)\bigr)dW_t^i\Bigr\rangle\\
&\quad +\|a(\Theta_{t,\tau}^{i,N},\rho_t^N)-a(\bar\Theta_{t,\tau}^i,\rho_t)\|^2\,dt.
\end{aligned}
\tag{Ito}
\end{equation}

By taking the expectation,

\begin{equation}
    \begin{aligned}
\frac{d}{dt}\mathbb E\|e_t^i\|^2
&=
2\mathbb E\Bigl\langle e_t^i,\,b(\Theta_{t,\tau}^{i,N},\rho_t^N)-b(\bar\Theta_{t,\tau}^i,\rho_t)\Bigr\rangle
+\mathbb E\|a(\Theta_{t,\tau}^{i,N},\rho_t^N)-a(\bar\Theta_{t,\tau}^i,\rho_t)\|^2.
\end{aligned}
\end{equation}

From the definition of $b(\cdot,\cdot)$,

\begin{align}
2\left\langle e_t^i,\;b(\Theta,\rho^N)-b(\bar\Theta,\rho)\right\rangle
&=
-2\lambda\langle e_t^i,\;e_t^i-(m_{\alpha,\beta,\tau}^{G,L}(\rho^N)-m_{\alpha,\beta,\tau}^{G,L}(\rho))\rangle\\
&=
-2\lambda\|e_t^i\|^2+2\lambda\langle e_t^i,\;m_{\alpha,\beta,\tau}^{G,L}(\rho^N)-m_{\alpha,\beta,\tau}^{G,L}(\rho)\rangle\\
&\le
-2\lambda\|e_t^i\|^2+2\lambda\|e_t^i\|\cdot \|m_{\alpha,\beta,\tau}^{G,L}(\rho^N)-m_{\alpha,\beta,\tau}^{G,L}(\rho)\|,\\
&\le
-\lambda\|e_t^i\|^2+\lambda \|m_{\alpha,\beta,\tau}^{G,L}(\rho^N)-m_{\alpha,\beta,\tau}^{G,L}(\rho)\|^2.
\end{align}

Then, from the definition of $a(\cdot,\cdot)$,

\begin{align}
    \|a(\Theta_{t,\tau}^{i,N},\rho_t^N)-a(\bar\Theta_{t,\tau}^i,\rho_t)\|^2
&=\sigma^2\|D(\Theta_{t,\tau}^{i,N}-m(\rho_t^N))-D(\bar\Theta_{t,\tau}^i-m(\rho_t))\|^2,\\
&\leq \sigma^2L_D^2\|e_t^i-m(\rho_t^N)+m(\rho_t)\|^2,\\
&\leq 2\sigma^2L_D^2\|e_t^i\|+2\sigma^2L_D^2\|m(\rho_t^N)-m(\rho_t)\|^2
\end{align}

where we apply the smoothness of $D(\cdot)$. As a result,

\begin{align}
\frac{d}{dt}\mathbb E\|e_t^i\|^2
&\le
\mathbb E\Bigl[-2\lambda\|e_t^i\|^2+\lambda\|e_t^i\|^2+\lambda\|m_{\alpha,\beta,\tau}^{G,L}(\rho_t^N)-m_{\alpha,\beta,\tau}^{G,L}(\rho_t)\|^2\Bigr]\\
&\quad +\mathbb E\Bigl[2\sigma^2 L_D^2\|e_t^i\|^2+2\sigma^2 L_D^2\|m_{\alpha,\beta,\tau}^{G,L}(\rho_t^N)-m_{\alpha,\beta,\tau}^{G,L}(\rho_t)\|^2\Bigr]\\
&=\Bigl(-\lambda+2\sigma^2 L_D^2\Bigr)\mathbb E\|e_t^i\|^2
+\Bigl(\lambda+2\sigma^2 L_D^2\Bigr)\mathbb E\|m_{\alpha,\beta,\tau}^{G,L}(\rho_t^N)-m_{\alpha,\beta,\tau}^{G,L}(\rho_t)\|^2.
\label{eq:e_dyn}
\end{align}

To bound the $\|m_{\alpha,\beta,\tau}^{G,L}(\rho_t^N)-m_{\alpha,\beta,\tau}^{G,L}(\rho_t)\|^2$, we define

\[
m(\rho)=\frac{A(\rho)}{B(\rho)},
\]

where 
\begin{equation}
w(x):=e^{-\alpha G(x)},
\qquad
\eta_\rho(x):=s\!\left(\frac{q(\rho)-L(x)}{\tau}\right),    
\end{equation}

and

\begin{equation}
A(\rho):=\int x\,w(x)\eta_\rho(x)\,\rho(dx),
\qquad
B(\rho):=\int w(x)\eta_\rho(x)\,\rho(dx).    
\end{equation}

We decompose it into (Discrete particles continous dynamic vs mean field)

\begin{equation}
\|m(\rho_t^N)-m(\rho_t)\|^2
\le
2\|m(\rho_t^N)-m(\bar\rho_t^N)\|^2
+
2\|m(\bar\rho_t^N)-m(\rho_t)\|^2,    
\end{equation}
and bound each term separately. 
We further define

\begin{equation}
    F_\nu(q):=\int s\!\left(\frac{q-L(x)}{\tau}\right)\nu(dx)-\beta.
\end{equation}

and assume

\begin{equation}
\partial_q F_\nu(q(\nu))
=
\frac1\tau\int s'\!\left(\frac{q-L(x)}{\tau}\right)\nu(dx)
\ge \kappa_{M,\tau}.
\end{equation}

Take a simplified notation

\begin{equation}
    q_t^N:=q_{\beta,\tau}^L[\rho_t^N],\qquad \bar q_t^N:=q_{\beta,\tau}^L[\bar\rho_t^N].
\end{equation}

we have ($I_m$: particles in ball M)

\begin{equation}
\begin{aligned}
    |q_t^N-\bar q_t^N|I_M(t)
&\le
\frac{1}{\kappa_{M,\tau}}\left|
F_{\rho_t^N}(\bar q_t^N)-F_{\bar\rho_t^N}(\bar q_t^N)
\right|I_M(t),~(\text{see~\Cref{eq:mid_val_thm}})\\
&=
\left|\frac1N\sum_{j=1}^N
\left[
s\!\left(\frac{\bar q_t^N-L(\Theta_{t,\tau}^{j,N})}{\tau}\right)
-
s\!\left(\frac{\bar q_t^N-L(\bar\Theta_{t,\tau}^{j})}{\tau}\right)
\right]\right| I_M(t),~(\text{definition})\\
&\leq \frac1N\sum_{j=1}^N
\left|s\!\left(\frac{\bar q_t^N-L(\Theta_{t,\tau}^{j,N})}{\tau}\right)
-
s\!\left(\frac{\bar q_t^N-L(\bar\Theta_{t,\tau}^{j})}{\tau}\right)\right| I_M(t),\\
&\leq \frac{L_s}{N}\sum_{j=1}^N
\left|\frac{L(\bar\Theta_{t,\tau}^{j})-L(\Theta_{t,\tau}^{j,N})}{\tau}\right| I_M(t),~(s(\cdot)~\text{is Liptisch})\\
&
\le
\frac{L_sL_{L,M}}{\tau\kappa_{M,\tau}}
\frac1N\sum_{j=1}^N\|e_t^j\| I_M(t).~\text{liptsch to lower level function}
\end{aligned}
\end{equation}

Thus,
\begin{equation}
|q_t^N-\bar q_t^N|^2 I_M(t)
\le
C_{q,M,\tau}^2\,
\frac1N\sum_{j=1}^N\|e_t^j\|^2 I_M(t).
\end{equation}

where $C_{q,M,\tau}:=\frac{L_sL_{L,M}}{\tau\kappa_{M,\tau}},$.

Then, we define

\begin{equation}
    \phi_q(x):=x e^{-\alpha G(x)} s\!\left(\frac{q-L(x)}{\tau}\right),
\qquad
\psi_q(x):=e^{-\alpha G(x)} s\!\left(\frac{q-L(x)}{\tau}\right)\label{eq:num_denom_double_weight}
\end{equation}

We have,

\begin{equation}
\begin{aligned}
    \|\phi_{q_1}(x)-\phi_{q_2}(y)\|I_M(t)
&\le
\Bigl\|x e^{-\alpha G(x)}-y e^{-\alpha G(y)}\Bigr\|I_M(t)
+
\|y\| e^{-\alpha G(y)}
\left|
s\!\left(\frac{q_1-L(x)}{\tau}\right)
-
s\!\left(\frac{q_2-L(y)}{\tau}\right)
\right|I_M(t),\\
& \le
\|x-y\| e^{-\alpha G(x)}I_M(t)
+
\|y\|\,
\bigl|e^{-\alpha G(x)}-e^{-\alpha G(y)}\bigr|I_M(t)\\
&+\|y\| e^{-\alpha G(y)}\left(\frac{L_s}{\tau}|q_1-q_2|
+
\frac{L_s}{\tau}|L(x)-L(y)|\right)I_M(t),\\
& \leq 
e^{\alpha \bar G_M}\Bigl(1+M\alpha L_{G,M}\Bigr)\|x-y\|I_M(t)+Me^{\alpha \bar G_M}\left(
\frac{L_s}{\tau}|q_1-q_2|
+
\frac{L_sL_{L,M}}{\tau}\|x-y\|\right)I_M(t),\\
&\leq 
e^{\alpha \bar G_M}
\left(
1+M\alpha L_{G,M}+M\frac{L_s(1+L_{L,M})}{\tau}
\right)\bigl(\|x-y\|+|q_1-q_2|\bigr)I_M(t),\\
&=C_{\phi,M,\tau}\bigl(\|x-y\|+|q_1-q_2|\bigr)I_M(t)
\end{aligned}
\end{equation}

where $
C_{\phi,M,\tau}
:=
e^{\alpha \bar G_M}
\left(
1+M\alpha L_{G,M}+M\frac{L_s(1+L_{L,M})}{\tau}
\right)$ .

Following the same process,

\begin{equation}
\begin{aligned}
    |\psi_{q_1}(x)-\psi_{q_2}(y)|I_M(t)
    & \leq
\bigl|e^{-\alpha G(x)}-e^{-\alpha G(y)}\bigr|I_M(t)
+
e^{-\alpha G(y)}
\left|
s\!\left(\frac{q_1-L(x)}{\tau}\right)-s\!\left(\frac{q_2-L(y)}{\tau}\right)
\right|I_M(t),\\
&\le
e^{\alpha \bar G_M}
\left(
\alpha L_{G,M}+\frac{L_sL_{L,M}}{\tau}
\right)\|x-y\|
+
e^{\alpha \bar G_M}\frac{L_s}{\tau}|q_1-q_2|,\\
&\leq e^{\alpha \bar G_M}
\left(
\alpha L_{G,M}+\frac{L_s(1+L_{L,M})}{\tau}
\right)\bigl(\|x-y\|+|q_1-q_2|\bigr)I_M(t),\\
&=C_{\psi,M,\tau}\bigl(\|x-y\|+|q_1-q_2|\bigr)I_M(t).
\end{aligned}
\end{equation}

where $
C_{\psi,M,\tau}
:=
e^{\alpha \bar G_M}
\left(
\alpha L_{G,M}+\frac{L_s(1+L_{L,M})}{\tau}
\right)
$.

As a result,

\begin{equation}
\begin{aligned}
|A(\rho_t^N)-A(\bar\rho_t^N)|I_M(t)
&=
\frac1N\left|\sum_{j=1}^N
\Big(
\phi_{q_t^N}(\Theta_{t,\tau}^{j,N})
-
\phi_{\bar q_t^N}(\bar\Theta_{t,\tau}^{j})
\Big)\right|I_M(t),\\
&\leq
\frac{C_{\phi,M,\tau}}{N}
\sum_{j=1}^N
\bigl(\|e_t^j\|+|q_t^N-\bar q_t^N|\bigr) I_M(t).
\end{aligned}
\end{equation}

We square both side,

\begin{equation}
\begin{aligned}
|A(\rho_t^N)-A(\bar\rho_t^N)|^2 I_M(t)
&\le
2C_{\phi,M,\tau}^2
\left[
\left(\frac1N\sum_{j=1}^N \|e_t^j\|\right)^2
+
|q_t^N-\bar q_t^N|^2
\right] I_M(t),\\
&\leq
2C_{\phi,M,\tau}^2(1+C_{q,M,\tau}^2)\,
\frac1N\sum_{j=1}^N \|e_t^j\|^2 I_M(t).
\end{aligned}
\end{equation}

Same for $B$,

\begin{equation}
\begin{aligned}
    |B(\rho_t^N)-B(\bar\rho_t^N)|I_M(t)
&=
\frac1N\left |\sum_{j=1}^N
\Bigl(
\psi_{q_t^N}(\Theta_{t,\tau}^{j,N})-\psi_{\bar q_t^N}(\bar\Theta_{t,\tau}^j)
\Bigr)\right|I_M(t),\\
&
\le
C_{\psi,M,\tau}
\left[
\frac1N\sum_{j=1}^N (\|e_t^j\|
+
|q_t^N-\bar q_t^N|)
\right]I_M(t).
\end{aligned}
\end{equation}

which indicates

\begin{equation}
    |B(\rho_t^N)-B(\bar\rho_t^N)|^2 I_M(t)
\le
2C_{\psi,M,\tau}^2(1+C_{q,M,\tau}^2)\,
\frac1N\sum_{j=1}^N \|e_t^j\|^2 I_M(t).
\end{equation}

Notice that,

\begin{equation}
    m(\rho_t^N)-m(\bar\rho_t^N)
=
\frac{A(\rho_t^N)-A(\bar\rho_t^N)}{B(\rho_t^N)}
+
A(\bar\rho_t^N)\frac{B(\bar\rho_t^N)-B(\rho_t^N)}{B(\rho_t^N)B(\bar\rho_t^N)},
\end{equation}

\begin{equation}
    |A(\bar\rho_t^N)|
=
\left|
\frac1N\sum_{j=1}^N \phi_{\bar q_t^N}(\bar\Theta_{t,\tau}^j)
\right|
\le
\frac1N\sum_{j=1}^N
\|\bar\Theta_{t,\tau}^j\|e^{-\alpha G(\bar\Theta_{t,\tau}^j)}
s\!\left(\frac{\bar q_t^N-L(\bar\Theta_{t,\tau}^j)}{\tau}\right)
\le
M e^{\alpha \bar G_M}
=:a_M.
\end{equation}

%{\color{blue} make sure you define the correct boundedness event. and what is $\bar G_M$?}

and,

\begin{equation}
    B(\rho)
=
\int e^{-\alpha G(x)}\eta_\rho(x)\rho(dx)
\ge e^{-\alpha\bar G_M}\int \eta_\rho(x)\rho(dx)
=
\beta e^{-\alpha\bar G_M}
:=
b_M>0,
\end{equation}

we have

\begin{equation}
\begin{aligned}
\|m(\rho_t^N)-m(\bar\rho_t^N)\|^2 I_M(t)
&\le
2\frac{|A(\rho_t^N)-A(\bar\rho_t^N)|^2}{b_M^2}I_M(t)
+
2\frac{a_M^2|B(\rho_t^N)-B(\bar\rho_t^N)|^2}{b_M^4}I_M(t),\\
&
\le
4(1+C_{q,M,\tau}^2)
\left(
\frac{C_{\phi,M,\tau}^2}{b_M^2}
+
\frac{a_M^2 C_{\psi,M,\tau}^2}{b_M^4}
\right)
\frac1N\sum_{j=1}^N\|e_t^j\|^2 I_M(t),\\
&\le
C_{M,\alpha,\tau}^{\rm coup}
\frac1N\sum_{j=1}^N\|e_t^j\|^2 I_M(t).
\end{aligned}
\end{equation}

where $
C_{M,\alpha,\tau}^{\rm coup}
=
4(1+C_{q,M,\tau}^2)
\left(
\frac{C_{\phi,M,\tau}^2}{b_M^2}
+
\frac{a_M^2 C_{\psi,M,\tau}^2}{b_M^4}
\right).$

Then, we consider $
\mathbb E\!\left[\|m(\bar\rho_t^N)-m(\rho_t)\|^2 I_M(t)\right]$, we define

\begin{equation}
\begin{aligned}
F_t(q):&=\int s\!\left(\frac{q-L(x)}{\tau}\right)\rho_t(dx)-\beta,\\
F_t^N(q):&=\int s\!\left(\frac{q-L(x)}{\tau}\right)\bar\rho_t^N(dx)-\beta
=
\frac1N\sum_{j=1}^N s\!\left(\frac{q-L(\bar\Theta_{t,\tau}^j)}{\tau}\right)-\beta.
\end{aligned}
\end{equation}

We denote $q_t:=q_{\beta,\tau}^L[\rho_t], \bar q_t^N:=q_{\beta,\tau}^L[\bar\rho_t^N]$. Thus 

\begin{align}
  F_t(q_t)=0, F_t^N(\bar q_t^N)=0~(\text{definition})
\end{align}
which indicates

\begin{align}
  \underbrace{F_t^N(\bar q_t^N)}-F_t^N(q_t)&=\partial_q F_t^N(\xi_t^N)\,(\bar q_t^N-q_t)~(\text{middle value theorem})\\
                                           &=-\bigl(F_t^N(q_t)-\underbrace{F_t(q_t)}\bigr)\label{eq:mid_val_thm}
\end{align}

As $\partial_qF_t^N\ge \kappa_{M,\tau}$, we have

\begin{equation}
\begin{aligned}
|\bar q_t^N-q_t|\,I_M(t)
&\le
\frac{1}{\kappa_{M,\tau}}
|F_t^N(q_t)-\underbrace{F_t(q_t)}|\,I_M(t),\\
&\le 
\frac{1}{\kappa_{M,\tau}N}\left|\sum_{j=1}^N s\!\left(\frac{q_t-L(\bar\Theta_{t,\tau}^j)}{\tau}\right)
-
\beta\right|I_M(t)~(\text{definition})
\end{aligned}
\end{equation}
We square both side,

\begin{equation}
\begin{aligned}
    \mathbb E\bigl[|\bar q_t^N-q_t|^2 I_M(t)\bigr]
&\le
\frac{1}{\kappa_{M,\tau}^2N^2}\sum_{j=1}^N\left| s\!\left(\frac{q_t-L(\bar\Theta_{t,\tau}^j)}{\tau}\right)
-
\beta\right|^2I_M(t),\\
&\le \frac{1}{\kappa_{M,\tau}^2N}I_M(t).
\end{aligned}
\end{equation}

where we apply $\left|s\!\left(\frac{q_t-L(\bar\Theta_{t,\tau}^j)}{\tau}\right)-\beta\right|\leq 1$.

By definition, see~\Cref{eq:num_denom_double_weight}, note that different notations of $q$ correspond to solutions w.r.t.~fixed $\beta$ but different fields.
\[
\bar A_t^N=\frac{1}{N}\sum_{j=1}^N \phi_{\bar q_t^N}(\bar\Theta_{t,\tau}^j), \qquad
A_t=\mathbb E\big[\phi_{q_t}(\bar\Theta_{t,\tau})\big].
\]
\[
\bar B_t^N=\frac{1}{N}\sum_{j=1}^N \psi_{\bar q_t^N}(\bar\Theta_{t,\tau}^j), \qquad
B_t=\mathbb E\big[\psi_{q_t}(\bar\Theta_{t,\tau})\big].
\]
Hence,
\[
\bar A_t^N-A_t
=
\underbrace{\frac{1}{N}\sum_{j=1}^N\Big(\phi_{\bar q_t^N}(\bar\Theta_{t,\tau}^j)-\phi_{q_t}(\bar\Theta_{t,\tau}^j)\Big)}_{=:T_{A,1}}
+
\underbrace{\frac{1}{N}\sum_{j=1}^N\Big(\phi_{q_t}(\bar\Theta_{t,\tau}^j)-\mathbb E[\phi_{q_t}(\bar\Theta_{t,\tau})]\Big)}_{=:T_{A,2}~\text{expectation 0}},
\]
and therefore
\[
|\bar A_t^N-A_t|^2 \le 2|T_{A,1}|^2+2|T_{A,2}|^2.
\]
For the first term, for fixed \(x\in B_M\),
\[
\|\phi_{q_1}(x)-\phi_{q_2}(x)\|
\le C_{\phi,M,\tau}\,|q_1-q_2|,
\]
we obtain
\[
|T_{A,1}|\,I_M(t)\le C_{\phi,M,\tau}\,|\bar q_t^N-q_t|\,I_M(t).
\]
It follows that
\[
\mathbb E\big[|T_{A,1}|^2 I_M(t)\big]
\le
\frac{C_{\phi,M,\tau}^2}{\kappa_{M,\tau}^2\,N}.
\]
For the second term, define
\[
Y_{A,t}^j:=\phi_{q_t}(\bar\Theta_{t,\tau}^j)-\mathbb E\big[\phi_{q_t}(\bar\Theta_{t,\tau})\big].
\]
Then \(\{Y_{A,t}^j\}_{j=1}^N\) are i.i.d. centered random vectors, and thus
\[
\mathbb E\big[|T_{A,2}|^2 I_M(t)\big]
\le
\mathbb E|T_{A,2}|^2
=
\frac{1}{N^2}\sum_{j=1}^N \mathbb E|Y_{A,t}^j|^2
\le
\frac{\Sigma_{A,M,T}^2}{N},
\]
where
\[
\Sigma_{A,M,T}^2:=\sup_{t\in[0,T]}\mathbb E\Big|\phi_{q_t}(\bar\Theta_{t,\tau})-\mathbb E\big[\phi_{q_t}(\bar\Theta_{t,\tau})\big]\Big|^2.
\]
Combining the above estimates yields
\[
\mathbb E\big[\|\bar A_t^N-A_t\|^2 I_M(t)\big]
\le
\frac{1}{N}\left(\frac{2C_{\phi,M,\tau}^2}{\kappa_{M,\tau}^2}+2\Sigma_{A,M,T}^2\right)I_M(t).
\]

Following the same process, we can prove

\begin{equation}
\begin{aligned}
\mathbb E[|\bar B_t^N-B_t|^2 I_M(t)]
\le
\frac1N
\left(
\frac{2C_{\psi,M,\tau}^2}{\kappa_{M,\tau}^2}
+
2\Sigma_{B,M,T}^2
\right)I_M(t).
\end{aligned}
\end{equation}

As $m(\bar\rho_t^N)-m(\rho_t)
=
\frac{\bar A_t^N}{\bar B_t^N}-\frac{A_t}{B_t}
=
\frac{\bar A_t^N-A_t}{\bar B_t^N}
+
A_t\frac{B_t-\bar B_t^N}{B_t\bar B_t^N}$, by defining $A_{T,\max}=\sup_{t\in[0,T]}|A_t|$,

\begin{equation}
\begin{aligned}
        \mathbb{E}[\|m(\bar\rho_t^N)-m(\rho_t)\|^2 I_M(t)]
&\le
\mathbb{E}\left[2\frac{|\bar A_t^N-A_t|^2}{b_M^2}I_M(t)
+
2\frac{|A_t|^2}{b_M^4}|\bar B_t^N-B_t|^2I_M(t)\right],\\
&\le\frac{4}{b_M^2}
\left(
\frac{C_{\phi,M,\tau}^2}{\kappa_{M,\tau}^2}
+\Sigma_{A,M}^2
\right)\frac1N
+
\frac{4A_{T,\max}^2}{b_M^4}
\left(
\frac{C_{\psi,M,\tau}^2}{\kappa_{M,\tau}^2}
+\Sigma_{B,M}^2
\right)\frac1N,\\
&=
\frac{C_{M,\alpha,\tau}^{\rm emp}}{N},
\end{aligned}
\end{equation}

where $C_{M,\alpha,\tau}^{\rm emp}
=
\frac{4}{b_M^2}
\left(
\frac{C_{\phi,M,\tau}^2}{\kappa_{M,\tau}^2}
+\Sigma_{A,M}^2
\right)
+
\frac{4A_{T,\max}^2}{b_M^4}
\left(
\frac{C_{\psi,M,\tau}^2}{\kappa_{M,\tau}^2}
+\Sigma_{B,M}^2
\right)$

Overall, 

\begin{equation}
\begin{aligned}
    \mathbb E[\|m(\rho_t^N)-m(\rho_t)\|^2 I_M(t)]
\le
2C_{M,\alpha,\tau}^{\rm coup}\frac1N\sum_{j=1}^N\mathbb E[\|e_t^j\|^2I_M(t)]
+
\frac{2C_{M,\alpha,\tau}^{\rm emp}}{N}.
\end{aligned}
\end{equation}
Take this into~\Cref{eq:e_dyn}, 

\begin{align}
\frac{d}{dt}\mathbb E\|e_t^i\|^2
&\le
\mathbb E\Bigl[-2\lambda\|e_t^i\|^2+\lambda\|e_t^i\|^2+\lambda\|m_{\alpha,\beta,\tau}^{G,L}(\rho_t^N)-m_{\alpha,\beta,\tau}^{G,L}(\rho_t)\|^2\Bigr]\nonumber\\
&\quad +\mathbb E\Bigl[2\sigma^2 L_D^2\|e_t^i\|^2+2\sigma^2 L_D^2\|m_{\alpha,\beta,\tau}^{G,L}(\rho_t^N)-m_{\alpha,\beta,\tau}^{G,L}(\rho_t)\|^2\Bigr]\nonumber\\
&=\Bigl(-\lambda+2\sigma^2 L_D^2\Bigr)\mathbb E\|e_t^i\|^2
+\Bigl(\lambda+2\sigma^2 L_D^2\Bigr)\mathbb E\|m_{\alpha,\beta,\tau}^{G,L}(\rho_t^N)-m_{\alpha,\beta,\tau}^{G,L}(\rho_t)\|^2\nonumber
~(\Cref{eq:e_dyn}~\text{repeated})
\end{align}

\begin{theorem}[Grönwall's inequality]
Let $u, a, b \in C([t_0,T];\mathbb{R})$ with $b(t)\ge 0$ for all $t\in [t_0,T]$.
Assume that
\[
u(t) \le a(t) + \int_{t_0}^t b(s)\,u(s)\,ds,
\qquad t\in [t_0,T].
\]
Then
\[
u(t) \le a(t) + \int_{t_0}^t a(s)b(s)\exp\!\left(\int_s^t b(r)\,dr\right)\,ds,
\qquad t\in [t_0,T].
\]
In particular, if $a(t)\equiv C$ is constant, then
\[
u(t) \le C\exp\!\left(\int_{t_0}^t b(s)\,ds\right),
\qquad t\in [t_0,T].
\]
\end{theorem}

\begin{theorem}[Differential Grönwall inequality]
Let $u \in C^1([t_0,T])$ and let $\beta \in C([t_0,T])$ with
\[
u'(t) \le \beta(t)u(t), \qquad t\in [t_0,T].
\]
Then
\[
u(t) \le u(t_0)\exp\!\left(\int_{t_0}^t \beta(s)\,ds\right),
\qquad t\in [t_0,T].
\]
\end{theorem}

\begin{theorem}[Grönwall's inequality (constant coefficient)]
Let $u:[t_0,T]\to \mathbb{R}$ be continuous and suppose that
\[
u(t) \le C + K\int_{t_0}^t u(s)\,ds,
\qquad t\in [t_0,T],
\]
where $C,K\ge 0$ are constants. Then
\[
u(t) \le C e^{K(t-t_0)},
\qquad t\in [t_0,T].
\]
\end{theorem}

%{\color{blue} Please write down again equation \eqref{eq:e_dyn} with the above bound and then apply the G theorem on that.}, 
via Grönwell's theorem, we get
$$
\max_{1\le i\le N}\mathbb E[\|e_t^i\|^2I_M(t)]
\le
\frac{C_{M,\alpha,\tau,T}}{N}.
$$

\textbf{The third term of \eqref{eq:terms}:} we need to show $\mathbb{E}\bigl[\|\widehat{\bar\Theta}_T^N-\widehat{\bar\Theta}_{T,0}^N\|_2^2 \mid \Omega_M\bigr]=\mathcal{O}(\tau^\gamma)$, where $\gamma>0$.

\begin{lemma}
If $\|f(x)-f(y)\|\le L\|x-y\|$, then
\begin{align}
\|\mathbb{E}_{\mu_1} f -\mathbb{E}_{\mu_2} f\| \le L\int \|x-y\|d\pi(x,y)
\end{align}
%{\color{blue} Where is $L$ in the above inequality? This resemble the Wasserstein distance. Please add the proofs of these lemmas.}
\end{lemma}

\begin{proof}
Let $\pi$ be any coupling of $\mu_1$ and $\mu_2$, so that its marginals are $\mu_1$ and $\mu_2$. Then
\begin{align}
\mathbb{E}_{\mu_1} f
&= \int f(x)\, d\mu_1(x)
= \int f(x)\, d\pi(x,y),
\\
\mathbb{E}_{\mu_2} f
&= \int f(y)\, d\mu_2(y)
= \int f(y)\, d\pi(x,y).
\end{align}
Hence,
\begin{align}
\mathbb{E}_{\mu_1} f - \mathbb{E}_{\mu_2} f
= \int \bigl(f(x)-f(y)\bigr)\, d\pi(x,y).
\end{align}
Taking norms and applying the triangle inequality,
\begin{align}
\left\|\mathbb{E}_{\mu_1} f - \mathbb{E}_{\mu_2} f\right\|
&=
\left\|\int \bigl(f(x)-f(y)\bigr)\, d\pi(x,y)\right\|
\\
&\le
\int \|f(x)-f(y)\|\, d\pi(x,y).
\end{align}
Since $f$ is $L$-Lipschitz,
\begin{align}
\|f(x)-f(y)\| \le L\|x-y\|.
\end{align}
Therefore,
\begin{align}
\left\|\mathbb{E}_{\mu_1} f - \mathbb{E}_{\mu_2} f\right\|
\le
L\int \|x-y\|\, d\pi(x,y).
\end{align}
\end{proof}

\begin{lemma}
If objective function $f$ is lower bounded by quadratic function
\begin{equation}
f  
\end{equation}
\[
\frac{e^{-\alpha f}}{\|\omega_f^\alpha\|_{L^1(\mu)}}
\leq
\exp\!\bigl(\alpha c_u(1+K)\bigr)
=: c_K .
\]
\end{lemma}
\begin{proof}
Jensen inequality gives

\[
\exp\!\left(\mathbb{E}(\cdot)\right)\leq \mathbb{E}\exp(\cdot)
\]
apply

\begin{align}\label{}
e^{-\alpha \int (f-\underline f)\,d\mu}
&\leq
\int e^{-\alpha(f-\underline f)}\,d\mu .
\end{align}
thus

\begin{align}\label{}
e^{-\alpha \int (f)\,d\mu} \cdot
e^{-\alpha \int (\underline f)\,d\mu}
&\leq
\int e^{-\alpha(f-\underline f)}\,d\mu .
\end{align}
\end{proof}

\begin{lemma}
Given objective function $f$,
  \begin{equation}
  |m_f[\mu]-m_f[\hat{\mu}] \le c_0W_2(\mu, \hat{\mu})
  \end{equation}
\end{lemma}

gbegin{proof}
\begin{align}\label{}
m_f[\mu]-m_f[\hat{\mu}]
=
\iint
\left[
\frac{x\,\omega_f^\alpha(x)}{\|\omega_f^\alpha\|_{L^1(\mu)}}
-
\frac{\hat{x}\,\omega_f^\alpha(\hat{x})}{\|\omega_f^\alpha\|_{L^1(\hat{\mu})}}
\right]
\,d\pi
:=
\iint \bigl(h(x)-h(\hat{x})\bigr)\,d\pi.
\end{align}

\begin{align}
h(x)-h(\hat{x})
&=
\frac{x\,\omega_f^\alpha(x)}{\|\omega_f^\alpha\|_{L^1(\mu)}}
-
\frac{\hat{x}\,\omega_f^\alpha(\hat{x})}{\|\omega_f^\alpha\|_{L^1(\hat{\mu})}}
\\
&=
\left(
\frac{x\,\omega_f^\alpha(x)}{\|\omega_f^\alpha\|_{L^1(\mu)}}
-
\underbrace{\frac{x\,\omega_f^\alpha(\hat{x})}{\|\omega_f^\alpha\|_{L^1(\mu)}}}
\right)
+
\left(
\frac{x\,\omega_f^\alpha(\hat{x})}{\|\omega_f^\alpha\|_{L^1(\mu)}}
-
\underbrace{\frac{\hat{x}\,\omega_f^\alpha(\hat{x})}{\|\omega_f^\alpha\|_{L^1(\mu)}}}
\right)
\\
&\qquad
+
\left(
\frac{\hat{x}\,\omega_f^\alpha(\hat{x})}{\|\omega_f^\alpha\|_{L^1(\mu)}}
-
\frac{\hat{x}\,\omega_f^\alpha(\hat{x})}{\|\omega_f^\alpha\|_{L^1(\hat{\mu})}}
\right)
\\
&=
\frac{x\bigl(\omega_f^\alpha(x)-\omega_f^\alpha(\hat{x})\bigr)}{\|\omega_f^\alpha\|_{L^1(\mu)}}
+
\frac{(x-\hat{x})\,\omega_f^\alpha(\hat{x})}{\|\omega_f^\alpha\|_{L^1(\mu)}}
+
\hat{x}\,\omega_f^\alpha(\hat{x})
\left(
\frac{1}{\|\omega_f^\alpha\|_{L^1(\mu)}}
-
\frac{1}{\|\omega_f^\alpha\|_{L^1(\hat{\mu})}}
\right)
\\
&=
\frac{x\bigl(\omega_f^\alpha(x)-\omega_f^\alpha(\hat{x})\bigr)}{\|\omega_f^\alpha\|_{L^1(\mu)}}
+
\frac{(x-\hat{x})\,\omega_f^\alpha(\hat{x})}{\|\omega_f^\alpha\|_{L^1(\mu)}}
+
\frac{\|\omega_f^\alpha\|_{L^1(\hat{\mu})}-\|\omega_f^\alpha\|_{L^1(\mu)}}
{\|\omega_f^\alpha\|_{L^1(\mu)}\,\|\omega_f^\alpha\|_{L^1(\hat{\mu})}}
\,\hat{x}\,\omega_f^\alpha(\hat{x})
\\
&=
\frac{(x-\hat{x})\,\omega_f^\alpha(\hat{x})}{\|\omega_f^\alpha\|_{L^1(\mu)}}
+
\frac{x\bigl(\omega_f^\alpha(x)-\omega_f^\alpha(\hat{x})\bigr)}{\|\omega_f^\alpha\|_{L^1(\mu)}}
+
\frac{\iint \bigl(\omega_f^\alpha(\hat{x})-\omega_f^\alpha(x)\bigr)\,d\pi}
{\|\omega_f^\alpha\|_{L^1(\mu)}\,\|\omega_f^\alpha\|_{L^1(\hat{\mu})}}
\,\hat{x}\,\omega_f^\alpha(\hat{x}).~(\text{Integration gives L1 norm})
\end{align}

%\end{proof}

\begin{lemma}
  Note that the dynamic is particles moving towards a time-varying attractor where the time varying attractor is calculated via a convex combination of particles where a first selection phase is based on $L$. Our soft selection mechanism let the \textbf{lumped up weight} behaves like a amplitude modulation signal of $L$ with tiny fluctuations caused by $G$: $w(\theta)=w_L(\theta)w_G(\theta)$ intead of $w(\theta)=w_L(\theta)\left(1+\epsilon w_G(\theta)\right)$.  
  So we have
  \begin{equation}
    \|w_L(\theta)w_G(\theta)\|_{\infty}\le\|w_L(\theta)\|_{\infty}\|w_G(\theta)\|_{\infty} 
  \end{equation}
  since weight is smaller than $1$, we have
  \begin{equation}
    \|w_L(\theta)w_G(\theta)\|_{\infty}\le \|w_G(\theta)\|_{\infty} 
  \end{equation}
  and
  \begin{equation}
    \|w_L(\theta)w_G(\theta)\|_{\infty}\le \|w_L(\theta)\|_{\infty} 
  \end{equation}
Now define the partition function $\eta^{(s)}(\rho, \alphaGs)=\langle w_L(\rho),w_G(\rho, \alphaGs) \rangle$ as an inner product be a functional of $\rho$, the partition function can be thought of a similarity measure between $G$ and $L$, but conditioned on the law $\rho$.
And 
\begin{align}
  m_{\alphaGs,\beta,\tau}^{G,L}(\rho) &= {\left\langle\frac{w_L(\rho, \alphaLs)w_G(\rho, \alphaGs)}{\langle w_L(\rho, \alphaLs),w_G(\rho, \alphaGs) \rangle}, \theta\right\rangle}_{\rho}\\
  m_{\alphaGh,\beta,\tau}^{G,L}(\rho) &= {\left\langle\frac{I_L(\rho, \beta) \cdot w_G(\rho, \alphaGh)}{\langle I_L(\rho, \beta),w_G(\rho, \alphaGh) \rangle}, \theta\right\rangle}_{\rho}
\end{align}
{\color{red}There are the same?}
Thus, under the same law $\rho$, for fixed $\alphaGh>> 1$ we can tune $\alphaGs, \alphaLs$, such that the tail distribution's particles' contribution to consensus calculation can be omitted with an error $O(\frac{1}{\alpha})$. Due to continuity of inner product operation, when we treat 
$w_L(\rho, \alphaLs)$ and $I_L(\rho, \beta)$ as two separate functional input, the difference of the inner product is bounded by $Cd\left(w_L(\rho, \alphaLs) \mid I_L(\rho, \beta)\right)$ where $C$ is a constant of the inner product's sensitivity to change of function. With $\alphaGs$ being large enough,
$d\left(w_L(\rho, \alphaLs) \mid I_L(\rho, \beta)\right)$ is bounded by $O(\frac{1}{\alphaLs})$
\label{lemma:consensus_point_functional}
\end{lemma}
{\color{red} What does this lemma say? }

Now we turn back to 
\begin{align}
{\|\widehat{\bar\Theta}_T^N-\widehat{\bar\Theta}_{T,0}^N\|}_2^2
\end{align}

First we do
\begin{align}
&\|m_{\alphaGs,\beta,\tau}^{G,L}(\rho^{(s)}) - m_{\alphaGh,\beta,0}^{G,L}(\rho^{(h)})\|\label{eq:m_s_rho_s_vs_m_h_r_h}\\
  =&\|m_{\alphaGs,\beta,\tau}^{G,L}(\rho^{(s)})-\underbrace{m_{\alphaGs,\beta,\tau}^{G,L}(\rho^{(h)})+m_{\alphaGs,\beta,\tau}^{G,L}(\rho^{(h)})}   - m_{\alphaGh,\beta,0}^{G,L}(\rho^{(h)})\|\label{eq:m_s_rho_s_vs_m_h_r_h_minus_m_s_rho_h}\\
\text{instead of}~&\|m_{\alphaGs,\beta,\tau}^{G,L}(\rho^{(s)})\underbrace{-m_{\alphaGh,\beta,0}^{G,L}(\rho^{(s)})+m_{\alphaGh,\beta,0}^{G,L}(\rho^{(s)})}   - m_{\alphaGh,\beta,0}^{G,L}(\rho^{(h)})\|\nonumber
\end{align}

Then using triangle inequality on~\Cref{eq:m_s_rho_s_vs_m_h_r_h_minus_m_s_rho_h}:

Note for law $\rho$, let $I(\theta, \beta)$ be indicator variable for selecting particles
\begin{align}
&\|m_{\alphaGs,\beta,\tau}^{G,L}(\rho)-m_{\alphaGh,\beta,0}^{G,L}(\rho)\|\\
=&\frac{\int \theta e^{-\alphaGs G(\theta)}\,s\!\left(\frac{q_{\beta,\tau}^L[\rho]-L(\theta)}{\tau}\right)\rho(d\theta)}{\int e^{-\alphaGs G(\theta)}\,s\!\left(\frac{q_{\beta,\tau}^L[\rho]-L(\theta)}{\tau}\right)\rho(d\theta)}- 
\frac{\int \theta I(\theta, \beta)e^{-\alphaGh G(\theta)}\rho(d\theta)}{\int e^{-\alphaGh I(\theta, \beta)G(\theta)}\rho(d\theta)}\\
=&O(\frac{1}{\alphaLs})~(\text{According to}~\Cref{lemma:consensus_point_functional})
\end{align}

Now it is left to show under the same consensus calculation mechanism, how the deviation of Law $\rho$ would result in different consensus point.
\begin{align}
&\|m_{\alphaGs,\beta,\tau}^{G,L}(\rho^{(s)})-m_{\alphaGs,\beta,\tau}^{G,L}(\rho^{(h)})\|\\
=&C_m d(\rho^{s} \mid \rho^{(h)})
\end{align}
The above inequality can be derived from Lemma 3.2 of~\cite{carrillo2018analytical}.

Now we have showed the consensus point discrepancy in~\Cref{eq:m_s_rho_s_vs_m_h_r_h} can be bounded.

$\ldots$ to be continued

\begin{remark}[to be done, skip for reading]
\begin{align}
  \|\langle w(\rho_1(t))\theta(\rho_1(t))\rangle-\langle w(\rho_2(t))\theta(\rho_2(t)) \rangle|\ &\le max_i |\theta^{(i)}_1-\theta_2^{(i)}\|\\
  &=\|\sum_i w^{(i)}_1\theta_1^{(i)}-\sum_i w^{(i)}_2\theta_2^{(i)}\|
\end{align}
note that $w^{(i)}-w^{(j)}\le L(\theta^{(i)}-\theta^{(j)})$

thus 

\begin{align}
\|\sum_i w^{(i)}_1\theta_1^{(i)}-\sum_i w^{(i)}_2\theta_2^{(i)}\|
&\le \sum_i \|w^{(i)}_1\theta_1^{(i)} -w^{(i)}_2\theta_2^{(i)}\|\\
&\le N \max_i
\end{align}
\end{remark}

%%%%%%%%%%%%%%%%%%%%%%%%%%%%%%%%%%%%%%%%%%%%%%%%%%%%%%%%%%%%%%%%%%%%%%%%%%%%%%%%%%%%%%%%%%%%%%%%%%%%%%%%%%%%%%%%%%%%%%%%%%%%%%%%%%%%%%%%%%%%%%%%%%%%%%%%%%%%%%%%%%%%%%

\begin{proposition}
\label{prop:soft-q2lp}
Let
\[
\Theta:=\arg\min_{\theta\in\mathbb{R}^d}L(\theta),
\qquad
L_\ast:=\min_{\theta\in\mathbb{R}^d}L(\theta),
\qquad
\theta^\ast:=\theta^\ast_{\mathrm{good}}.
\]
Let $\varrho\in\mathcal{P}(\mathbb{R}^d)$ satisfy
\[
\operatorname{supp}(\varrho)\subset B_R(0)
\]
for some $R>0$. For fixed $\beta\in(0,1]$ and $\tau>0$, let
\[
q=q_{\beta,\tau}^L[\varrho]
\]
be defined by
\[
\int_{\mathbb{R}^d} s\!\left(\frac{q-L(\theta)}{\tau}\right)\varrho(d\theta)=\beta,
\]
and define
\[
\eta_{\varrho,\tau}(\theta):=s\!\left(\frac{q-L(\theta)}{\tau}\right),
\qquad
J_{\beta,\tau}^L[\varrho](d\theta):=\eta_{\varrho,\tau}(\theta)\varrho(d\theta).
\]
Furthermore, define the soft consensus point
\[
m_{\alpha,\beta,\tau}^{G,L}(\varrho)
:=
\frac{\displaystyle\int_{\mathbb{R}^d}\theta e^{-\alpha G(\theta)}\,dJ_{\beta,\tau}^L[\varrho](\theta)}
{\displaystyle\int_{\mathbb{R}^d}e^{-\alpha G(\theta)}\,dJ_{\beta,\tau}^L[\varrho](\theta)}.
\]

Assume that the following hold.

\medskip

\noindent
(i) The selector $s:\mathbb{R}\to[0,1]$ is nondecreasing.

\medskip

\noindent
(ii) There exist constants $H_L>0$ and $h_L\in(0,1]$ such that
\[
|L(x)-L(y)|\le H_L\|x-y\|_2^{h_L}
\qquad
\forall x,y\in B_R(0).
\]

\medskip

\noindent
(iii) There exist constants $\eta_L>0$, $\nu_L>0$, and $L_\infty>0$ such that
\[
\operatorname{dist}(x,\Theta)\le \frac{1}{\eta_L}(L(x)-L_\ast)^{\nu_L}
\qquad
\text{whenever }L(x)-L_\ast\le L_\infty.
\]

\medskip

\noindent
(iv) There exist constants $r_G>0$, $\eta_G>0$, $\nu_G>0$, and $G_\infty>0$ such that
\[
\|x-\theta^\ast\|_2\le \frac{1}{\eta_G}\bigl(G(x)-G(\theta^\ast)\bigr)^{\nu_G}
\]
for every $x\in N_{r_G}(\Theta)$ satisfying $G(x)-G(\theta^\ast)\le G_\infty$.

\medskip

\noindent
(v) There exists $\delta_q>0$ such that
\[
q+\delta_q\le L_\ast+\min\Bigl\{L_\infty,(\eta_L r_G)^{1/\nu_L}\Bigr\}.
\]

\medskip

\noindent
(vi) Let $r>0$ be such that $B_r(\theta^\ast)\subset B_R(0)$, and define
\[
G_r:=\sup_{\theta\in B_r(\theta^\ast)}\bigl(G(\theta)-G(\theta^\ast)\bigr),
\qquad
\Delta_{G,R,r}:=\sup_{\theta\in B_r(\theta^\ast)}G(\theta)-\inf_{x\in B_R(0)}G(x).
\]
Assume in addition that $u>0$ is chosen so that
\[
u+G_r\le G_\infty.
\]

Set
\[
c_{\mathrm{in}}
:=
s\!\left(\frac{q-L_\ast-H_Lr^{h_L}}{\tau}\right),
\qquad
c_{\mathrm{out}}
:=
s\!\left(-\frac{\delta_q}{\tau}\right).
\]
%{\color{blue}Is this to bound the Fourth term of \eqref{eq:terms}?}
Then
\[
\bigl\|m_{\alpha,\beta,\tau}^{G,L}(\varrho)-\theta^\ast\bigr\|_2
\le
\frac{(u+G_r)^{\nu_G}}{\eta_G}
+
\frac{e^{-\alpha u}}{c_{\mathrm{in}}\varrho(B_r(\theta^\ast))}
\int_{\mathbb{R}^d}\|\theta-\theta^\ast\|_2\,dJ_{\beta,\tau}^L[\varrho](\theta)
+
\frac{2R\,e^{\alpha\Delta_{G,R,r}}\,c_{\mathrm{out}}}
{c_{\mathrm{in}}\varrho(B_r(\theta^\ast))}.
\]
\end{proposition}

\begin{proof}
For notational simplicity, write
\[
J:=J_{\beta,\tau}^L[\varrho],
\qquad
m:=m_{\alpha,\beta,\tau}^{G,L}(\varrho),
\qquad
\eta(\theta):=\eta_{\varrho,\tau}(\theta).
\]

We divide the proof into four steps.

\medskip

\noindent
\textbf{Step 1: Lower bound on the soft weight inside $B_r(\theta^\ast)$.}
Let $\theta\in B_r(\theta^\ast)$. Since $B_r(\theta^\ast)\subset B_R(0)$ and $L(\theta^\ast)=L_\ast$, the Hölder continuity of $L$ on $B_R(0)$ yields
\[
L(\theta)-L_\ast
\le H_L\|\theta-\theta^\ast\|_2^{h_L}
\le H_L r^{h_L}.
\]
Hence
\[
q-L(\theta)\ge q-L_\ast-H_Lr^{h_L}.
\]
Since $s$ is nondecreasing, we obtain
\[
\eta(\theta)
=
s\!\left(\frac{q-L(\theta)}{\tau}\right)
\ge
s\!\left(\frac{q-L_\ast-H_Lr^{h_L}}{\tau}\right)
=
c_{\mathrm{in}}.
\]
Therefore,
\[
J(B_r(\theta^\ast))
=
\int_{B_r(\theta^\ast)}\eta(\theta)\,\varrho(d\theta)
\ge
c_{\mathrm{in}}\varrho(B_r(\theta^\ast)).
\tag{1}
\label{eq:soft-q2lp-mass-in}
\]

\medskip

\noindent
\textbf{Step 2: Upper bound on the soft weight outside $N_{r_G}(\Theta)$.}
Let $\theta\notin N_{r_G}(\Theta)$. Then $\operatorname{dist}(\theta,\Theta)>r_G$. By the inverse continuity property of $L$, this implies
\[
L(\theta)-L_\ast\ge (\eta_L r_G)^{1/\nu_L}.
\]
Indeed, if $L(\theta)-L_\ast<(\eta_L r_G)^{1/\nu_L}$, then in particular $L(\theta)-L_\ast\le L_\infty$ and thus
\[
\operatorname{dist}(\theta,\Theta)
\le
\frac{1}{\eta_L}(L(\theta)-L_\ast)^{\nu_L}
<
r_G,
\]
which is a contradiction.

Using assumption (v), we therefore obtain
\[
q-L(\theta)
\le
L_\ast+(\eta_L r_G)^{1/\nu_L}-\delta_q-L(\theta)
\le
-\delta_q.
\]
By monotonicity of $s$,
\[
\eta(\theta)
=
s\!\left(\frac{q-L(\theta)}{\tau}\right)
\le
s\!\left(-\frac{\delta_q}{\tau}\right)
=
c_{\mathrm{out}}.
\tag{2}
\label{eq:soft-q2lp-mass-out}
\]

\medskip

\noindent
\textbf{Step 3: Lower bound on the normalization factor.}
Set
\[
\underline{G}_R:=\inf_{x\in B_R(0)}G(x),
\qquad
\overline{G}(\theta):=G(\theta)-\underline{G}_R.
\]
Since $\operatorname{supp}(\varrho)\subset B_R(0)$, we have $\overline{G}(\theta)\ge 0$ on $\operatorname{supp}(\varrho)$, and
\[
m
=
\frac{\displaystyle\int_{\mathbb{R}^d}\theta e^{-\alpha \overline{G}(\theta)}\,dJ(\theta)}
{\displaystyle\int_{\mathbb{R}^d}e^{-\alpha \overline{G}(\theta)}\,dJ(\theta)}.
\]
Let
\[
Z:=\int_{\mathbb{R}^d}e^{-\alpha \overline{G}(\theta)}\,dJ(\theta).
\]
Then by \eqref{eq:soft-q2lp-mass-in},
\[
Z
\ge
\int_{B_r(\theta^\ast)}e^{-\alpha \overline{G}(\theta)}\,dJ(\theta)
\ge
e^{-\alpha \sup_{B_r(\theta^\ast)}\overline{G}}\,J(B_r(\theta^\ast))
\ge
e^{-\alpha \Delta_{G,R,r}}\,c_{\mathrm{in}}\varrho(B_r(\theta^\ast)).
\tag{3}
\label{eq:soft-q2lp-Z-lower}
\]

\medskip

\noindent
\textbf{Step 4: Decomposition of the consensus integral.}
Define
\[
r_e:=\frac{(u+G_r)^{\nu_G}}{\eta_G}.
\]
Then
\[
m-\theta^\ast
=
\frac{1}{Z}\int_{\mathbb{R}^d}(\theta-\theta^\ast)e^{-\alpha\overline{G}(\theta)}\,dJ(\theta).
\]
Hence, by splitting the integral into three regions,
\[
\|m-\theta^\ast\|_2
\le T_1+T_2+T_3,
\]
where
\[
T_1
:=
\frac{1}{Z}\int_{B_{r_e}(\theta^\ast)}
\|\theta-\theta^\ast\|_2 e^{-\alpha\overline{G}(\theta)}\,dJ(\theta),
\]
\[
T_2
:=
\frac{1}{Z}\int_{N_{r_G}(\Theta)\setminus B_{r_e}(\theta^\ast)}
\|\theta-\theta^\ast\|_2 e^{-\alpha\overline{G}(\theta)}\,dJ(\theta),
\]
\[
T_3
:=
\frac{1}{Z}\int_{N_{r_G}(\Theta)^c}
\|\theta-\theta^\ast\|_2 e^{-\alpha\overline{G}(\theta)}\,dJ(\theta).
\]

We estimate these terms one by one.

\medskip

\noindent
\emph{Estimate for $T_1$.}
On $B_{r_e}(\theta^\ast)$ we have $\|\theta-\theta^\ast\|_2\le r_e$, hence
\[
T_1
\le
r_e
=
\frac{(u+G_r)^{\nu_G}}{\eta_G}.
\tag{4}
\label{eq:soft-q2lp-T1}
\]

\medskip

\noindent
\emph{Estimate for $T_2$.}
Let $\theta\in N_{r_G}(\Theta)\setminus B_{r_e}(\theta^\ast)$. Then
\[
\|\theta-\theta^\ast\|_2>r_e.
\]
By the inverse continuity property of $G$ on $N_{r_G}(\Theta)$, this implies
\[
G(\theta)-G(\theta^\ast)>u+G_r.
\]
Indeed, otherwise we would have
\[
\|\theta-\theta^\ast\|_2
\le
\frac{1}{\eta_G}\bigl(G(\theta)-G(\theta^\ast)\bigr)^{\nu_G}
\le
\frac{(u+G_r)^{\nu_G}}{\eta_G}
=
r_e,
\]
a contradiction.

Now let $\xi\in B_r(\theta^\ast)$. By the definition of $G_r$,
\[
G(\xi)-G(\theta^\ast)\le G_r.
\]
Therefore,
\[
G(\theta)-G(\xi)\ge u,
\]
and hence
\[
\overline{G}(\theta)-\sup_{\xi\in B_r(\theta^\ast)}\overline{G}(\xi)\ge u.
\]
Equivalently,
\[
e^{-\alpha \overline{G}(\theta)}
\le
e^{-\alpha u}e^{-\alpha \sup_{B_r(\theta^\ast)}\overline{G}}.
\]
Using \eqref{eq:soft-q2lp-Z-lower}, we obtain
\[
T_2
\le
\frac{e^{-\alpha u}}{c_{\mathrm{in}}\varrho(B_r(\theta^\ast))}
\int_{N_{r_G}(\Theta)\setminus B_{r_e}(\theta^\ast)}
\|\theta-\theta^\ast\|_2\,dJ(\theta)
\]
and thus
\[
T_2
\le
\frac{e^{-\alpha u}}{c_{\mathrm{in}}\varrho(B_r(\theta^\ast))}
\int_{\mathbb{R}^d}\|\theta-\theta^\ast\|_2\,dJ(\theta).
\tag{5}
\label{eq:soft-q2lp-T2}
\]

\medskip

\noindent
\emph{Estimate for $T_3$.}
Since $\operatorname{supp}(\varrho)\subset B_R(0)$ and $\theta^\ast\in B_R(0)$, we have
\[
\|\theta-\theta^\ast\|_2\le 2R
\qquad
\forall \theta\in\operatorname{supp}(\varrho).
\]
Moreover, by \eqref{eq:soft-q2lp-mass-out}, for every $\theta\in N_{r_G}(\Theta)^c$,
\[
\eta(\theta)\le c_{\mathrm{out}}.
\]
Since $\overline{G}\ge 0$, it follows that
\[
\int_{N_{r_G}(\Theta)^c}
\|\theta-\theta^\ast\|_2 e^{-\alpha\overline{G}(\theta)}\,dJ(\theta)
\le
2R\,c_{\mathrm{out}}.
\]
Using again \eqref{eq:soft-q2lp-Z-lower}, we obtain
\[
T_3
\le
\frac{2R\,c_{\mathrm{out}}}{e^{-\alpha\Delta_{G,R,r}}\,c_{\mathrm{in}}\varrho(B_r(\theta^\ast))}
=
\frac{2R\,e^{\alpha\Delta_{G,R,r}}\,c_{\mathrm{out}}}
{c_{\mathrm{in}}\varrho(B_r(\theta^\ast))}.
\tag{6}
\label{eq:soft-q2lp-T3}
\]

Combining \eqref{eq:soft-q2lp-T1}, \eqref{eq:soft-q2lp-T2}, and \eqref{eq:soft-q2lp-T3} concludes the proof.
\end{proof}

\begin{theorem}
\label{thm:soft-mf-convergence}
Let $\rho=(\rho_t)_{t\ge 0}\subset \mathcal{P}_2(\mathbb{R}^d)$ be a weak solution of the soft mean-field dynamics associated with the consensus map $m_{\alpha,\beta,\tau}^{G,L}$, and define
\[
V(t):=\frac12 W_2^2(\rho_t,\delta_{\theta^\ast}),
\qquad
\theta^\ast:=\theta^\ast_{\mathrm{good}}.
\]
Assume that
\[
a:=2\lambda-d\sigma^2>0,
\qquad
b:=\sqrt{2}\,(\lambda+d\sigma^2),
\qquad
c:=\frac{d\sigma^2}{2}.
\]

Assume furthermore that the following hold.

\medskip

\noindent
(i) For almost every $t\ge 0$,
\[
\dot V(t)
\le
-aV(t)+b\sqrt{V(t)}\,M(t)+c\,M(t)^2,
\]
where
\[
M(t):=\bigl\|m_{\alpha,\beta,\tau}^{G,L}(\rho_t)-\theta^\ast\bigr\|_2.
\]

\medskip

\noindent
(ii) For every finite horizon $T>0$, there exist constants
\[
r>0,\quad r_G>0,\quad u>0,\quad m_\ast>0,\quad \underline{c}_{\mathrm{in}}>0,\quad \overline{c}_{\mathrm{out}}(\tau)\ge 0
\]
such that, for all $t\in[0,T]$,
\[
\rho_t(B_r(\theta^\ast))\ge m_\ast,
\]
and, writing
\[
q_t:=q_{\beta,\tau}^L[\rho_t],
\qquad
\eta_t(\theta):=s\!\left(\frac{q_t-L(\theta)}{\tau}\right),
\]
we have
\[
\eta_t(\theta)\ge \underline{c}_{\mathrm{in}}
\quad
\forall \theta\in B_r(\theta^\ast),
\qquad
\eta_t(\theta)\le \overline{c}_{\mathrm{out}}(\tau)
\quad
\forall \theta\in N_{r_G}(\Theta)^c.
\]

\medskip

\noindent
(iii) The hypotheses of Proposition~\ref{prop:soft-q2lp} hold uniformly on $[0,T]$ with the same constants $r$, $r_G$, and $u$.

Set
\[
G_r:=\sup_{\theta\in B_r(\theta^\ast)}\bigl(G(\theta)-G(\theta^\ast)\bigr),
\qquad
\Delta_{G,R,r}:=\sup_{\theta\in B_r(\theta^\ast)}G(\theta)-\inf_{x\in B_R(0)}G(x),
\]
and define
\[
A:=\frac{(u+G_r)^{\nu_G}}{\eta_G},
\qquad
B:=\frac{\sqrt{2}\,e^{-\alpha u}}{\underline{c}_{\mathrm{in}}m_\ast},
\qquad
\Lambda_\tau:=\frac{2R\,e^{\alpha\Delta_{G,R,r}}\overline{c}_{\mathrm{out}}(\tau)}
{\underline{c}_{\mathrm{in}}m_\ast}.
\]

Then the following statements hold.

\medskip

\noindent
\textbf{(a) Residual convergence for fixed $\tau$.}
For almost every $t\in[0,T]$,
\[
\dot V(t)
\le
-\bigl(a-bB-cB^2\bigr)V(t)
+
\bigl(b+2cB\bigr)(A+\Lambda_\tau)\sqrt{V(t)}
+
c(A+\Lambda_\tau)^2.
\tag{1}
\label{eq:soft-main-diff-ineq}
\]
In particular, if
\[
\kappa:=a-bB-cB^2>0,
\]
then
\[
V(t)
\le
e^{-\kappa t/2}V(0)
+
\frac{2}{\kappa}
\left(
c+\frac{(b+2cB)^2}{2\kappa}
\right)
(A+\Lambda_\tau)^2
\qquad
\forall t\in[0,T].
\]

\medskip

\noindent
\textbf{(b) Finite-accuracy convergence.}
Let $\varepsilon>0$ and $\vartheta\in(0,1)$ be given. Assume that the parameters are chosen so that
\[
bB+cB^2
+
\sqrt{\frac{2}{\varepsilon}}\,(b+2cB)(A+\Lambda_\tau)
+
\frac{2c}{\varepsilon}(A+\Lambda_\tau)^2
\le
\vartheta a.
\tag{2}
\label{eq:soft-smallness-condition}
\]
Define the hitting time
\[
\tau_\varepsilon
:=
\inf\left\{
t\ge 0:\,
V(t)\le \frac{\varepsilon}{2}
\right\}.
\]
Then, for every $t\in[0,\tau_\varepsilon]$,
\[
V(t)\le V(0)e^{-(1-\vartheta)a t}.
\]
Consequently,
\[
\tau_\varepsilon
\le
\frac{1}{(1-\vartheta)a}
\log\!\left(\frac{2V(0)}{\varepsilon}\right),
\]
and therefore
\[
W_2^2(\rho_{\tau_\varepsilon},\delta_{\theta^\ast})\le \varepsilon.
\]
In particular, for
\[
T_\varepsilon
:=
\frac{1}{(1-\vartheta)a}
\log\!\left(\frac{2V(0)}{\varepsilon}\right),
\]
one has
\[
W_2^2(\rho_{T_\varepsilon},\delta_{\theta^\ast})\le \varepsilon.
\]
\end{theorem}

\begin{proof}
Fix a finite horizon $T>0$. For $t\in[0,T]$, apply Proposition~\ref{prop:soft-q2lp} with $\varrho=\rho_t$. By assumption (ii),
\[
\rho_t(B_r(\theta^\ast))\ge m_\ast,
\qquad
\eta_t(\theta)\ge \underline{c}_{\mathrm{in}}
\ \text{on } B_r(\theta^\ast),
\qquad
\eta_t(\theta)\le \overline{c}_{\mathrm{out}}(\tau)
\ \text{on } N_{r_G}(\Theta)^c.
\]
Hence
\[
M(t)
\le
A
+
\frac{e^{-\alpha u}}{\underline{c}_{\mathrm{in}}m_\ast}
\int_{\mathbb{R}^d}\|\theta-\theta^\ast\|_2\,dJ_t(\theta)
+
\Lambda_\tau,
\]
where
\[
J_t(d\theta):=\eta_t(\theta)\rho_t(d\theta).
\]
Since $0\le \eta_t\le 1$, we have $J_t\le \rho_t$ as measures, and therefore
\[
\int_{\mathbb{R}^d}\|\theta-\theta^\ast\|_2\,dJ_t(\theta)
\le
\int_{\mathbb{R}^d}\|\theta-\theta^\ast\|_2\,d\rho_t(\theta).
\]
By Cauchy--Schwarz,
\[
\int_{\mathbb{R}^d}\|\theta-\theta^\ast\|_2\,d\rho_t(\theta)
\le
\left(
\int_{\mathbb{R}^d}\|\theta-\theta^\ast\|_2^2\,d\rho_t(\theta)
\right)^{1/2}
=
\sqrt{2V(t)}.
\]
Thus
\[
M(t)\le A+B\sqrt{V(t)}+\Lambda_\tau.
\tag{3}
\label{eq:soft-M-bound}
\]

Substituting \eqref{eq:soft-M-bound} into assumption (i), we obtain
\[
\dot V(t)
\le
-aV(t)
+
b\sqrt{V(t)}\bigl(A+B\sqrt{V(t)}+\Lambda_\tau\bigr)
+
c\bigl(A+B\sqrt{V(t)}+\Lambda_\tau\bigr)^2.
\]
Expanding and regrouping terms gives
\[
\dot V(t)
\le
-\bigl(a-bB-cB^2\bigr)V(t)
+
\bigl(b+2cB\bigr)(A+\Lambda_\tau)\sqrt{V(t)}
+
c(A+\Lambda_\tau)^2,
\]
which is exactly \eqref{eq:soft-main-diff-ineq}. This proves part (a) up to the residual estimate.

Assume now that $\kappa:=a-bB-cB^2>0$. Then \eqref{eq:soft-main-diff-ineq} yields
\[
\dot V(t)
\le
-\kappa V(t)
+
\bigl(b+2cB\bigr)(A+\Lambda_\tau)\sqrt{V(t)}
+
c(A+\Lambda_\tau)^2.
\]
By Young's inequality,
\[
\bigl(b+2cB\bigr)(A+\Lambda_\tau)\sqrt{V(t)}
\le
\frac{\kappa}{2}V(t)
+
\frac{(b+2cB)^2}{2\kappa}(A+\Lambda_\tau)^2.
\]
Therefore,
\[
\dot V(t)
\le
-\frac{\kappa}{2}V(t)
+
\left(
c+\frac{(b+2cB)^2}{2\kappa}
\right)(A+\Lambda_\tau)^2.
\]
An application of Gr\"onwall's inequality gives
\[
V(t)
\le
e^{-\kappa t/2}V(0)
+
\frac{2}{\kappa}
\left(
c+\frac{(b+2cB)^2}{2\kappa}
\right)(A+\Lambda_\tau)^2,
\]
which proves part (a).

We now prove part (b). Let
\[
\tau_\varepsilon
:=
\inf\left\{
t\ge 0:\,
V(t)\le \frac{\varepsilon}{2}
\right\}.
\]
Fix $t\in[0,\tau_\varepsilon]$. Then for almost every $s\in[0,t]$ we have
\[
V(s)\ge \frac{\varepsilon}{2}.
\]
Hence
\[
\sqrt{V(s)}\le \sqrt{\frac{2}{\varepsilon}}\,V(s)
\qquad\text{and}\qquad
1\le \frac{2}{\varepsilon}V(s).
\]
Using these two inequalities in \eqref{eq:soft-main-diff-ineq}, we obtain
\[
\dot V(s)
\le
-\Biggl[
a-bB-cB^2
-
\sqrt{\frac{2}{\varepsilon}}(b+2cB)(A+\Lambda_\tau)
-
\frac{2c}{\varepsilon}(A+\Lambda_\tau)^2
\Biggr]V(s).
\]
By the smallness condition \eqref{eq:soft-smallness-condition},
\[
\dot V(s)\le -(1-\vartheta)a\,V(s)
\qquad
\text{for a.e. }s\in[0,\tau_\varepsilon].
\]
Integrating this differential inequality yields
\[
V(t)\le V(0)e^{-(1-\vartheta)a t}
\qquad
\forall t\in[0,\tau_\varepsilon].
\]
In particular, if
\[
T_\varepsilon
:=
\frac{1}{(1-\vartheta)a}
\log\!\left(\frac{2V(0)}{\varepsilon}\right),
\]
then
\[
V(T_\varepsilon)\le \frac{\varepsilon}{2}.
\]
By the definition of $\tau_\varepsilon$, this implies $\tau_\varepsilon\le T_\varepsilon$, and therefore
\[
W_2^2(\rho_{\tau_\varepsilon},\delta_{\theta^\ast})
=
2V(\tau_\varepsilon)
\le
\varepsilon.
\]
Since $V(T_\varepsilon)\le \varepsilon/2$ as well, we also have
\[
W_2^2(\rho_{T_\varepsilon},\delta_{\theta^\ast})\le \varepsilon.
\]
This concludes the proof.
\end{proof}
