# Supplementary material for: Convergence of Consensus-Based Particle Methods for Nonconvex Bi-Level Optimization
Source: arXiv:2605.19667 source file (2026-05-19)
Supplement: Supplementary file 2 [file appendix1.tex]

\section{Problem, notation, and primitive assumptions}

\subsection{Soft quantile and consensus point}

Fix $\alpha>0$, $\beta\in(0,1)$, and $\tau>0$. For $\rho\in\Pcal(\R^d)$, the soft $\beta$-quantile $q^L_{\beta,\tau}[\rho]$ is the unique solution of
\begin{equation}
    \int_{\R^d} s\left(\frac{q-L(x)}{\tau}\right)\rho(\dd x)=\beta.
    \label{eq:soft_quantile_def}
\end{equation}
When no confusion is possible, we write $q_\rho:=q^L_{\beta,\tau}[\rho]$. Define
\begin{equation}
    \eta_{\rho,\tau}(x):=s\left(\frac{q_\rho-L(x)}{\tau}\right),
    \qquad
    J^L_{\beta,\tau}[\rho](\dd x):=\eta_{\rho,\tau}(x)\rho(\dd x).
\end{equation}
Then
{\color{red} Is there an integral missing here?}
\begin{equation}
    J^L_{\beta,\tau}[\rho](\R^d)=\beta.
    \label{eq:J_mass_beta}
\end{equation}
Set $w_\alpha(x):=e^{-\alpha G(x)}$ and
\begin{equation}
    A(\rho):=\int_{\R^d}xw_\alpha(x)\,\dd J^L_{\beta,\tau}[\rho](x),
    \qquad
    B(\rho):=\int_{\R^d}w_\alpha(x)\,\dd J^L_{\beta,\tau}[\rho](x).
\end{equation}
The soft consensus point is
\begin{equation}
    m(\rho):=m^{G,L}_{\alpha,\beta,\tau}(\rho):=\frac{A(\rho)}{B(\rho)}.
\end{equation}

\subsection{Particle systems and diffusion structure}

Throughout the paper, the matrix-valued diffusion coefficient is fixed as
\begin{equation}
    D(z):=\norm{z}_2\Id,
    \qquad z\in\R^d.
    \label{eq:D_def}
\end{equation}
Consequently,
\begin{equation}
    D(z)D(z)^\top=\norm{z}_2^2\Id,
    \qquad
    \Tr\big(D(z)D(z)^\top\big)=d\norm{z}_2^2,
    \qquad
    \norm{D(z)-D(y)}_F\le \sqrt d\norm{z-y}_2.
    \label{eq:D_identities}
\end{equation}
The interacting particle system is
\begin{equation}
    \dd\Theta^{i,N}_{t,\tau}
    =-\lambda\big(\Theta^{i,N}_{t,\tau}-m(\rho^{N,{\rm int}}_{t,\tau})\big)\dd t
    +\sigma D\big(\Theta^{i,N}_{t,\tau}-m(\rho^{N,{\rm int}}_{t,\tau})\big)\dd W^i_t,
    \label{eq:interacting_sde}
\end{equation}
where
\begin{equation}
    \rho^{N,{\rm int}}_{t,\tau}:=\frac1N\sum_{i=1}^N\delta_{\Theta^{i,N}_{t,\tau}}.
\end{equation}
The mean-field process is
\begin{equation}
    \dd\Theta_{t,\tau}
    =-\lambda\big(\Theta_{t,\tau}-m(\rho_{t,\tau})\big)\dd t
    +\sigma D\big(\Theta_{t,\tau}-m(\rho_{t,\tau})\big)\dd W_t,
    \qquad
    \rho_{t,\tau}:=\Law(\Theta_{t,\tau}).
    \label{eq:mf_sde}
\end{equation}
Let $\bar\Theta^1_{t,\tau},\dots,\bar\Theta^N_{t,\tau}$ denote i.i.d. copies of the mean-field process, synchronously coupled with the interacting system through the same initial data and Brownian motions. Define
\begin{equation}
    \bar\rho^N_{t,\tau}:=\frac1N\sum_{i=1}^N\delta_{\bar\Theta^i_{t,\tau}}.
\end{equation}
The Euler--Maruyama scheme with $K\Delta t=T$ is
\begin{equation}
    \theta^i_{k+1,\tau}
    =\theta^i_{k,\tau}
    -\lambda\Delta t\big(\theta^i_{k,\tau}-m(\rho^N_{k,\tau})\big)
    +\sigma\sqrt{\Delta t}\,D\big(\theta^i_{k,\tau}-m(\rho^N_{k,\tau})\big)B^i_k,
    \label{eq:em_scheme}
\end{equation}
where $B^i_k\sim N(0,\Id)$ are i.i.d. and
\begin{equation}
    \rho^N_{k,\tau}:=\frac1N\sum_{i=1}^N\delta_{\theta^i_{k,\tau}}.
\end{equation}

\subsection{Primitive assumptions}

\begin{assumption}[Primitive assumptions]\label{ass:primitive}
The following conditions hold.
\begin{enumerate}
    \item \textbf{Parameters and selector.} The parameters satisfy
    \begin{equation}
        \alpha>0,
        \qquad
        \beta\in(0,1),
        \qquad
        \tau>0,
        \qquad
        \lambda>0,
        \qquad
        \sigma>0.
    \end{equation}
    The selector $s:\R\to(0,1)$ is $C^1$, strictly increasing, and Lipschitz continuous with Lipschitz constant $L_s$. Moreover,
    \begin{equation}
        \lim_{z\to-\infty}s(z)=0,
        \qquad
        \lim_{z\to+\infty}s(z)=1.
    \end{equation}
    There exists $C_->0$ such that
    \begin{equation}
        s(-z)\le C_-e^{-z},
        \qquad z\ge0.
        \label{eq:s_left_tail}
    \end{equation}

    \item \textbf{Lower-level objective.} The function $L$ is globally Lipschitz with constant $L_L$. There exist $\eta_L>0$, $\nu_L>0$, and $L_\infty>0$ such that
    \begin{equation}
        \dist(x,\Theta)\le \eta_L^{-1}\big(L(x)-L^\star\big)^{\nu_L}
        \quad\text{whenever } L(x)-L^\star\le L_\infty.
        \label{eq:L_error_bound}
    \end{equation}

    \item \textbf{Upper-level objective.} The function $G$ is globally Lipschitz with constant $L_G$ and bounded from below:
    \begin{equation}
        G(x)\ge G_{\min},
        \qquad x\in\R^d.
        \label{eq:G_lower_bound}
    \end{equation}
    We write
    \begin{equation}
        G_0^+:=\max\{G(0),0\}.
        \label{eq:G0plus_def}
    \end{equation}
    Hence global Lipschitz continuity implies the positive-part growth bound
    \begin{equation}
        G_+(x):=\max\{G(x),0\}
        \le G_0^+ + L_G\norm{x}_2,
        \qquad x\in\R^d.
        \label{eq:G_positive_growth}
    \end{equation}

 There exists a deterministic constant $C_m>0$ such that every proof-relevant measure $\rho$ appearing in the moment estimates for the interacting and mean-field dynamics satisfies
    \begin{equation}
        \norm{m(\rho)}_2^4
        \le C_m^4\int_{\R^d}\norm{x}_2^4\rho(\dd x).
        \label{eq:consensus_moment_stability}
    \end{equation}
    More explicitly, \eqref{eq:consensus_moment_stability} is required for $\rho=\rho^{N,{\rm int}}_{t,\tau}$ and $\rho=\rho_{t,\tau}$ on every finite horizon used below. This assumption replaces the older global upper bound $G\le G_{\max}$; it is the only place where the fourth-moment estimate is closed.

    There exists $R_G>0$ such that for every $r_G\in(0,R_G]$ there is
    \begin{equation}
        \tilde\theta_{r_G}\in N_{r_G}(\Theta)\cap B_{r_G}(\theta^\star),
        \qquad
        G(\tilde\theta_{r_G})=\min_{x\in N_{r_G}(\Theta)}G(x).
        \label{eq:G_local_min}
    \end{equation}
    Moreover, there exist $\eta_G>0$, $\nu_G>0$, and $G_\infty>0$, independent of $r_G$, such that
    \begin{equation}
        \norm{x-\tilde\theta_{r_G}}_2
        \le \eta_G^{-1}\big(G(x)-G(\tilde\theta_{r_G})\big)^{\nu_G}
        \label{eq:G_error_bound}
    \end{equation}
    whenever $x\in N_{r_G}(\Theta)$ and $G(x)-G(\tilde\theta_{r_G})\le G_\infty$.

    \item \textbf{Initialization.} The initial law satisfies $\rho_0\in\Pcal_4(\R^d)$. We write
    \begin{equation}
        \mu_4:=\int_{\R^d}\norm{x}_2^4\rho_0(\dd x)<\infty.
        \label{eq:mu4_def}
    \end{equation}

    \item 
\label{ass:weak-mf-solution}
For every finite horizon \(T>0\), the mean-field equation
\[
d\Theta_{t,\tau}
=
-\lambda\bigl(\Theta_{t,\tau}-m(\rho_{t,\tau})\bigr)\,dt
+
\sigma D\bigl(\Theta_{t,\tau}-m(\rho_{t,\tau})\bigr)\,dW_t,
\qquad
\rho_{t,\tau}:=\Law(\Theta_{t,\tau}),
\]
admits a weak solution on \([0,T]\). We assume that this solution has continuous
paths, finite fourth moments, and that its law satisfies the associated weak
Fokker--Planck formulation.

    % \item \textbf{Well-posedness and weak formulation.} For every finite horizon $T>0$ and every $N\in\N$, the interacting system \eqref{eq:interacting_sde}, the i.i.d. mean-field copies of \eqref{eq:mf_sde}, and the Euler scheme \eqref{eq:em_scheme} are defined on a common filtered probability space with continuous SDE paths. The mean-field law $\rho_{t,\tau}$ satisfies the Fokker--Planck weak formulation associated with \eqref{eq:mf_sde} for all $C_c^2$ test functions, and all fourth moments appearing below are finite, and the map $t\mapsto V_\tau(t):=\frac12\int\norm{x-\theta^\star}_2^2\rho_{t,\tau}(\dd x)$ is continuous on every finite horizon.
\end{enumerate}
\end{assumption}

\begin{lemma}[Existence and uniqueness of the soft quantile]\label{lem:quantile_existence}
Under Assumption~\ref{ass:primitive}(A1), for every $\rho\in\Pcal(\R^d)$, equation \eqref{eq:soft_quantile_def} has a unique solution.
\end{lemma}

\begin{proof}
For fixed $\rho$, define
\begin{equation}
    H_\rho(q):=\int_{\R^d}s\left(\frac{q-L(x)}{\tau}\right)\rho(\dd x).
\end{equation}
Since $0<s<1$ and $s$ is continuous, dominated convergence implies that $H_\rho$ is continuous. The limits of $s$ imply
\begin{equation}
    \lim_{q\to-\infty}H_\rho(q)=0,
    \qquad
    \lim_{q\to+\infty}H_\rho(q)=1.
\end{equation}
Because $\beta\in(0,1)$, the intermediate value theorem gives existence. If $q_2>q_1$, then strict monotonicity of $s$ gives
\begin{equation}
    s\left(\frac{q_2-L(x)}{\tau}\right)
    >s\left(\frac{q_1-L(x)}{\tau}\right)
    \qquad\forall x\in\R^d.
\end{equation}
Integrating yields $H_\rho(q_2)>H_\rho(q_1)$, hence the solution is unique.
\end{proof}

\section{Quantile inverse stability from local strong monotonicity}

For $\nu\in\Pcal(\R^d)$ define
\begin{equation}
    F_\nu(q):=\int_{\R^d}s\left(\frac{q-L(x)}{\tau}\right)\nu(\dd x)-\beta.
    \label{eq:F_nu_def}
\end{equation}

\begin{assumption}[Uniform local strong monotonicity of the soft quantile map]\label{ass:quantile_monotonicity}
Fix a finite horizon $T>0$ and a cutoff level $M>0$. Let
\begin{equation}
    \mathfrak M_{T,M}^N
    :=\left\{\rho_{t,\tau}:t\in[0,T]\right\}
    \cup\left\{\bar\rho^N_{t,\tau}:t\in[0,T]\right\}
    \cup\left\{\rho^{N,{\rm int}}_{t\wedge\tau_M,\tau}:t\in[0,T]\right\}.
    \label{eq:measure_family_quantile}
\end{equation}
For every
$\nu\in\mathfrak M_{T,M}^N$ and every $q$ lying between $q_\nu$ and any other quantile $q_\mu$ with
$\mu\in\mathfrak M_{T,M}^N$, the following two-sided local monotonicity inequality holds:
\begin{equation}
    \big(F_\nu(q)-F_\nu(q_\nu)\big)(q-q_\nu)
    \ge \kappa |q-q_\nu|^2.
    \label{eq:uniform_local_strong_monotonicity}
\end{equation}
Equivalently, for such $q$,
\begin{align}
    F_\nu(q)-F_\nu(q_\nu)&\ge \kappa(q-q_\nu), && q\ge q_\nu,\label{eq:strong_mono_right}\\
    F_\nu(q_\nu)-F_\nu(q)&\ge \kappa(q_\nu-q), && q\le q_\nu.\label{eq:strong_mono_left}
\end{align}
\end{assumption}

Note that 
$$
F_\nu(q_\nu)=0
$$

So we need specific $s$ function that make the above inequality true. But then you need the above assumption for $\kappa$ to be nonzero for all $\nu\in \mathfrak M_{T,M}^N$. 
for example $s$ could be sigmoid and other functions.

% \begin{remark}
% The one-sided inequality \eqref{eq:strong_mono_right} alone is not sufficient to control
% $|q_\mu-q_\nu|$ for arbitrary pairs $\mu,\nu$, because the case $q_\mu<q_\nu$ requires the left-side
% inequality \eqref{eq:strong_mono_left}. Assumption~\ref{ass:quantile_monotonicity} is therefore the
% minimal symmetric finite-difference form needed for the absolute-value inverse stability used below.
% \end{remark}

\begin{lemma}[Inverse stability under uniform local strong monotonicity]\label{lem:inverse_stability}
Assume Assumption~\ref{ass:quantile_monotonicity}. For every $\mu,\nu\in\mathfrak M_{T,M}^N$,
\begin{equation}
    |q_\mu-q_\nu|
    \le \kappa^{-1}|F_\mu(q_\nu)-F_\nu(q_\nu)|.
    \label{eq:inverse_stability_result}
\end{equation}
\end{lemma}

\begin{proof}
Since $F_\mu(q_\mu)=0$ and $F_\nu(q_\nu)=0$, one has
\begin{equation}
    |F_\mu(q_\nu)-F_\nu(q_\nu)|=|F_\mu(q_\nu)|.
    \label{eq:inverse_stability_start}
\end{equation}
If $q_\nu\le q_\mu$, then \eqref{eq:strong_mono_left} applied to $F_\mu$ with $q=q_\nu$ gives
\begin{equation}
    F_\mu(q_\mu)-F_\mu(q_\nu)
    \ge \kappa(q_\mu-q_\nu).
    \label{eq:inverse_case_left}
\end{equation}
Because $F_\mu(q_\mu)=0$, \eqref{eq:inverse_case_left} yields
\begin{equation}
    |F_\mu(q_\nu)|=-F_\mu(q_\nu)
    \ge \kappa(q_\mu-q_\nu).
\end{equation}
If $q_\nu>q_\mu$, then \eqref{eq:strong_mono_right} applied to $F_\mu$ with $q=q_\nu$ gives
\begin{equation}
    F_\mu(q_\nu)-F_\mu(q_\mu)
    \ge \kappa(q_\nu-q_\mu).
    \label{eq:inverse_case_right}
\end{equation}
Again $F_\mu(q_\mu)=0$, so
\begin{equation}
    |F_\mu(q_\nu)|=F_\mu(q_\nu)
    \ge \kappa(q_\nu-q_\mu).
\end{equation}
Combining the two cases with \eqref{eq:inverse_stability_start} proves \eqref{eq:inverse_stability_result}.
\end{proof}

\section{Deterministic bounds and cutoff event}

For $R_4>0$ define the moment-dependent denominator and numerator constants
\begin{equation}
    b(R_4):=\beta\exp\left[-\frac{\alpha}{\beta}\left(G_0^+ + L_GR_4^{1/4}\right)\right],
    \qquad
    a(R_4):=\beta^{1/2}e^{-\alpha G_{\min}}R_4^{1/4}.
    \label{eq:baR_def}
\end{equation}
The following lemma is the replacement for the old bound $B(\rho)\ge \beta e^{-\alpha G_{\max}}$.

\begin{lemma}[Moment-dependent denominator and numerator bounds]\label{lem:moment_denominator_bound}
Let $\rho\in\Pcal_4(\R^d)$ satisfy
\begin{equation}
    \int_{\R^d}\norm{x}_2^4\rho(\dd x)\le R_4.
    \label{eq:R4_assumption}
\end{equation}
Then
\begin{equation}
    B(\rho)\ge b(R_4),
    \qquad
    \norm{A(\rho)}_2\le a(R_4).
    \label{eq:B_A_moment_bounds}
\end{equation}
\end{lemma}

\begin{proof}
Let $J:=J^L_{\beta,\tau}[\rho]$. By \eqref{eq:J_mass_beta}, the measure
\begin{equation}
    \mu_J(\dd x):=\beta^{-1}J(\dd x)
\end{equation}
is a probability measure. Since $z\mapsto e^{-\alpha z}$ is convex, Jensen's inequality gives
\begin{align}
    B(\rho)
    &=\int e^{-\alpha G(x)}J(\dd x)                                      \\
    &=\beta\int e^{-\alpha G(x)}\mu_J(\dd x)                              \\
    &\ge \beta\exp\left(-\alpha\int G(x)\mu_J(\dd x)\right).             \label{eq:B_jensen_moment_proof}
\end{align}
Because $G(x)\le G_+(x)$ and $J\le \rho$ as measures,
\begin{align}
    \int G(x)\mu_J(\dd x)
    &\le \int G_+(x)\mu_J(\dd x)                                          \\
    &=\beta^{-1}\int G_+(x)J(\dd x)                                        \\
    &\le \beta^{-1}\int G_+(x)\rho(\dd x).                                \label{eq:G_muJ_positive_bound}
\end{align}
Using \eqref{eq:G_positive_growth}, Cauchy's inequality, and \eqref{eq:R4_assumption},
\begin{align}
    \int G_+(x)\rho(\dd x)
    &\le G_0^+ + L_G\int \norm{x}_2\rho(\dd x)                              \\
    &\le G_0^+ + L_G\left(\int\norm{x}_2^4\rho(\dd x)\right)^{1/4}          \\
    &\le G_0^+ + L_GR_4^{1/4}.                                                \label{eq:G_positive_moment_bound}
\end{align}
Combining \eqref{eq:B_jensen_moment_proof}, \eqref{eq:G_muJ_positive_bound}, and \eqref{eq:G_positive_moment_bound} yields $B(\rho)\ge b(R_4)$.

For the numerator, the lower bound $G\ge G_{\min}$ gives
\begin{align}
    \norm{A(\rho)}_2
    &\le e^{-\alpha G_{\min}}\int \norm{x}_2J(\dd x)                       \\
    &\le e^{-\alpha G_{\min}}\left(\int\norm{x}_2^2J(\dd x)\right)^{1/2}J(\R^d)^{1/2} \\
    &\le e^{-\alpha G_{\min}}\left(\int\norm{x}_2^2\rho(\dd x)\right)^{1/2}\beta^{1/2} \\
    &\le \beta^{1/2}e^{-\alpha G_{\min}}R_4^{1/4}=a(R_4).
\end{align}
This proves \eqref{eq:B_A_moment_bounds}.
\end{proof}

The fourth-moment estimates below do not use the denominator bound \eqref{eq:B_A_moment_bounds}. They use only the consensus-moment stability assumption \eqref{eq:consensus_moment_stability}; this separation is what avoids a circular argument.

\subsection{Cutoff event and stopped-process inequality}

For $M>0$, set
\begin{equation}
    \mathcal M_T
    :=\sup_{t\in[0,T]}\frac1N\sum_{i=1}^N
    \max\left\{\norm{\Theta^{i,N}_{t,\tau}}_2^4,\norm{\bar\Theta^i_{t,\tau}}_2^4\right\},
    \qquad
    \Omega_M:=\{\mathcal M_T\le M\}.
\end{equation}
Define the cutoff time
\begin{equation}
    \tau_M
    :=\inf\left\{t\in[0,T]:
    \frac1N\sum_{i=1}^N
    \max\left\{\norm{\Theta^{i,N}_{t,\tau}}_2^4,\norm{\bar\Theta^i_{t,\tau}}_2^4\right\}>M\right\},
    \label{eq:tau_M_def}
\end{equation}
with the convention $\tau_M=T$ if the set is empty. Let
\begin{equation}
    I_M(t):=\1_{\{t\le \tau_M\}}.
    \label{eq:IM_def}
\end{equation}
Then $I_M(T)=\1_{\Omega_M}$ and $I_M(T)\le I_M(t)$ for $t\le T$.

\begin{lemma}[Stopped integral inequality]\label{lem:stopped_integral_ineq}
Let $\tau$ be a stopping time and let $Y_t\ge0$ be a continuous adapted process with $Y_0=0$. Suppose that for some progressively measurable process $f_t$ with $\int_0^T\E|f_t|\dd t<\infty$, the stopped process satisfies
\begin{equation}
    Y_{t\wedge\tau}
    \le \int_0^t \1_{\{s\le\tau\}}f_s\dd s+M_{t\wedge\tau},
    \qquad t\in[0,T],
    \label{eq:stopped_process_ineq}
\end{equation}
where $M_{t\wedge\tau}$ is a true martingale with zero expectation. Then
\begin{equation}
    \E\big[Y_t\1_{\{t\le\tau\}}\big]
    \le \int_0^t\E\big[f_s\1_{\{s\le\tau\}}\big]\dd s,
    \qquad t\in[0,T].
    \label{eq:stopped_integral_conclusion}
\end{equation}
If the right-hand side is absolutely continuous in $t$, this is equivalent to the distributional differential inequality
\begin{equation}
    \frac{\dd}{\dd t}\E\big[Y_t\1_{\{t\le\tau\}}\big]
    \le \E\big[f_t\1_{\{t\le\tau\}}\big].
    \label{eq:stopped_differential_conclusion}
\end{equation}
\end{lemma}

\begin{proof}
Because $Y_t\ge0$,
\begin{equation}
    Y_t\1_{\{t\le\tau\}}\le Y_{t\wedge\tau}.
\end{equation}
Taking expectations in \eqref{eq:stopped_process_ineq} and using $\E M_{t\wedge\tau}=0$ gives
\begin{equation}
    \E\big[Y_t\1_{\{t\le\tau\}}\big]
    \le \E Y_{t\wedge\tau}
    \le \int_0^t\E\big[f_s\1_{\{s\le\tau\}}\big]\dd s.
\end{equation}
This proves \eqref{eq:stopped_integral_conclusion}. The distributional differential form follows by differentiating the absolutely continuous upper bound.
\end{proof}

\subsection{Fourth-moment boundedness with explicit constants}

Let $B_{4,d}$ be any fixed BDG constant such that, for every continuous $d$-dimensional stochastic integral $M_t=\int_0^t H_s\dd W_s$,
\begin{equation}
    \E\sup_{t\le T}\norm{M_t}_2^4
    \le B_{4,d}\E\left(\int_0^T\norm{H_s}_F^2\dd s\right)^2.
    \label{eq:BDG_constant}
\end{equation}
Define
\begin{equation}
    K_{\rm bd}(T)
    :=216(1+C_m^4)\left(\lambda^4T^3+\sigma^4B_{4,d}d^2T\right),
    \label{eq:Kbd_def}
\end{equation}
\begin{equation}
    C_{\rm bd}(T):=54\mu_4\exp\big(K_{\rm bd}(T)T\big).
    \label{eq:Cbd_def}
\end{equation}

\begin{lemma}[Fourth-moment bound]\label{lem:moment_bound}
Under Assumption~\ref{ass:primitive}, for every $T>0$,
\begin{equation}
    \E[\mathcal M_T]\le C_{\rm bd}(T),
    \qquad
    \Prob(\Omega_M^c)\le \frac{C_{\rm bd}(T)}{M}.
    \label{eq:moment_and_cutoff_bound}
\end{equation}
\end{lemma}

\begin{proof}
For the interacting system set $m^N_t:=m(\rho^{N,{\rm int}}_{t,\tau})$. For fixed $i$,
\begin{equation}
    \Theta^{i,N}_{t,\tau}
    =\Theta^{i,N}_{0,\tau}
    -\lambda\int_0^t(\Theta^{i,N}_{s,\tau}-m^N_s)\dd s
    +\sigma\int_0^tD(\Theta^{i,N}_{s,\tau}-m^N_s)\dd W^i_s.
\end{equation}
Using $(a+b+c)^4\le27(a^4+b^4+c^4)$ gives
\begin{align}
    \E\sup_{t\le T}\norm{\Theta^{i,N}_{t,\tau}}_2^4
    &\le 27\E\norm{\Theta^{i,N}_{0,\tau}}_2^4                                                     \\
    &\quad +27\lambda^4\E\sup_{t\le T}\norm{\int_0^t(\Theta^{i,N}_{s,\tau}-m^N_s)\dd s}_2^4        \\
    &\quad +27\sigma^4\E\sup_{t\le T}\norm{\int_0^tD(\Theta^{i,N}_{s,\tau}-m^N_s)\dd W^i_s}_2^4.
    \label{eq:moment_start}
\end{align}
Jensen's inequality in time gives
\begin{equation}
    \sup_{t\le T}\norm{\int_0^t(\Theta^{i,N}_{s,\tau}-m^N_s)\dd s}_2^4
    \le T^3\int_0^T\norm{\Theta^{i,N}_{s,\tau}-m^N_s}_2^4\dd s.
    \label{eq:drift_jensen}
\end{equation}
By $(a+b)^4\le8(a^4+b^4)$ and the consensus-moment stability bound \eqref{eq:consensus_moment_stability},
\begin{equation}
    \norm{\Theta^{i,N}_{s,\tau}-m^N_s}_2^4
    \le 8\norm{\Theta^{i,N}_{s,\tau}}_2^4
    +8C_m^4\frac1N\sum_{j=1}^N\norm{\Theta^{j,N}_{s,\tau}}_2^4.
    \label{eq:theta_minus_m_fourth}
\end{equation}
For the stochastic integral, \eqref{eq:BDG_constant}, Cauchy's inequality in time, and \eqref{eq:D_identities} imply
\begin{align}
    \E\sup_{t\le T}\norm{\int_0^tD(\Theta^{i,N}_{s,\tau}-m^N_s)\dd W^i_s}_2^4
    &\le B_{4,d}\E\left(\int_0^T\norm{D(\Theta^{i,N}_{s,\tau}-m^N_s)}_F^2\dd s\right)^2       \\
    &=B_{4,d}\E\left(\int_0^Td\norm{\Theta^{i,N}_{s,\tau}-m^N_s}_2^2\dd s\right)^2              \\
    &\le B_{4,d}d^2T\int_0^T\E\norm{\Theta^{i,N}_{s,\tau}-m^N_s}_2^4\dd s.
    \label{eq:diffusion_bdg}
\end{align}
Define
\begin{equation}
    U_N(t):=\frac1N\sum_{i=1}^N\E\sup_{u\le t}\norm{\Theta^{i,N}_{u,\tau}}_2^4.
\end{equation}
Averaging \eqref{eq:moment_start} over $i$, using \eqref{eq:drift_jensen}, \eqref{eq:theta_minus_m_fourth}, \eqref{eq:diffusion_bdg}, and
\begin{equation}
    \E\norm{\Theta^{i,N}_{s,\tau}}_2^4
    \le \E\sup_{u\le s}\norm{\Theta^{i,N}_{u,\tau}}_2^4,
\end{equation}
we obtain
\begin{equation}
    U_N(T)
    \le 27\mu_4+K_{\rm bd}(T)\int_0^T U_N(s)\dd s.
\end{equation}
Gronwall's inequality gives
\begin{equation}
    U_N(T)\le 27\mu_4\exp\big(K_{\rm bd}(T)T\big).
    \label{eq:interacting_moment_final}
\end{equation}
For the i.i.d. mean-field copies, the same proof applies. Indeed, $m(\rho_{s,\tau})$ satisfies
\begin{equation}
    \norm{m(\rho_{s,\tau})}_2^4
    \le C_m^4\E\norm{\bar\Theta^1_{s,\tau}}_2^4,
\end{equation}
and hence
\begin{equation}
    \bar U_N(T):=\frac1N\sum_{i=1}^N\E\sup_{u\le T}\norm{\bar\Theta^i_{u,\tau}}_2^4
    \le 27\mu_4\exp\big(K_{\rm bd}(T)T\big).
    \label{eq:mf_copy_moment_final}
\end{equation}
Since $\max\{a,b\}\le a+b$, \eqref{eq:interacting_moment_final} and \eqref{eq:mf_copy_moment_final} imply
\begin{equation}
    \E[\mathcal M_T]
    \le 54\mu_4\exp\big(K_{\rm bd}(T)T\big)=C_{\rm bd}(T).
\end{equation}
Markov's inequality gives $\Prob(\Omega_M^c)\le C_{\rm bd}(T)/M$.
\end{proof}

\section{Moment-based soft Laplace principle}

\begin{proposition}[Soft quantitative quantiled Laplace principle without compact support]\label{prop:laplace_no_compact}
Assume Assumption~\ref{ass:primitive}. Let $\varrho\in\Pcal_2(\R^d)$, $q=q^L_{\beta,\tau}[\varrho]$, and $J=J^L_{\beta,\tau}[\varrho]$. Assume that for some $r_G\in(0,R_G]$, $r\in(0,r_G]$, $u>0$, and $\delta_q>0$,
\begin{equation}
    q+\delta_q
    \le L^\star+\min\left\{L_\infty,(\eta_Lr_G)^{1/\nu_L}\right\},
    \label{eq:laplace_q_condition}
\end{equation}
\begin{equation}
    \varrho(B_r(\theta^\star))>0,
    \qquad
    u+\widetilde G_r\le G_\infty,
    \label{eq:laplace_other_conditions}
\end{equation}
where
\begin{equation}
    \tilde\theta_G:=\tilde\theta_{r_G},
    \qquad
    \widetilde G_r:=\sup_{\theta\in B_r(\theta^\star)}\big(G(\theta)-G(\tilde\theta_G)\big),
    \qquad
    \Delta_r:=\sup_{\theta\in B_r(\theta^\star)}G(\theta)-G_{\min}.
\end{equation}
Set
\begin{equation}
    c_{\rm in}(q,r):=s\left(\frac{q-L^\star-L_Lr}{\tau}\right),
    \qquad
    c_{\rm out}(\delta_q):=s\left(-\frac{\delta_q}{\tau}\right).
\end{equation}
Then
\begin{align}
    \norm{m(\varrho)-\theta^\star}_2
    &\le r_G+\frac{(u+\widetilde G_r)^{\nu_G}}{\eta_G}                                                   \\
    &\quad +\frac{e^{-\alpha u}}{c_{\rm in}(q,r)\varrho(B_r(\theta^\star))}
    \int_{\R^d}\norm{\theta-\tilde\theta_G}_2\dd J(\theta)                                                \\
    &\quad +\frac{e^{\alpha\Delta_r}c_{\rm out}(\delta_q)}{c_{\rm in}(q,r)\varrho(B_r(\theta^\star))}
    \int_{\R^d}\norm{\theta-\tilde\theta_G}_2\varrho(\dd\theta).
    \label{eq:laplace_first_bound}
\end{align}
If
\begin{equation}
    V_\varrho:=\frac12\int_{\R^d}\norm{\theta-\theta^\star}_2^2\varrho(\dd\theta),
\end{equation}
then
\begin{align}
    \norm{m(\varrho)-\theta^\star}_2
    &\le r_G+\frac{(u+\widetilde G_r)^{\nu_G}}{\eta_G}
    +\frac{e^{-\alpha u}}{c_{\rm in}(q,r)\varrho(B_r(\theta^\star))}
    \big(\sqrt{2V_\varrho}+\beta r_G\big)                                                  \\
    &\quad
    +\frac{e^{\alpha\Delta_r}c_{\rm out}(\delta_q)}{c_{\rm in}(q,r)\varrho(B_r(\theta^\star))}
    \big(\sqrt{2V_\varrho}+r_G\big).
    \label{eq:laplace_V_bound}
\end{align}
\end{proposition}

\begin{proof}
Write $m=m(\varrho)$, $\eta=\eta_{\varrho,\tau}$, and $\tilde\theta=\tilde\theta_G$.

First, if $\theta\in B_r(\theta^\star)$, then global Lipschitz continuity of $L$ gives
\begin{equation}
    L(\theta)-L^\star\le L_L\norm{\theta-\theta^\star}_2\le L_Lr.
\end{equation}
Thus
\begin{equation}
    \eta(\theta)
    =s\left(\frac{q-L(\theta)}{\tau}\right)
    \ge s\left(\frac{q-L^\star-L_Lr}{\tau}\right)
    =c_{\rm in}(q,r),
\end{equation}
and therefore
\begin{equation}
    J(B_r(\theta^\star))
    \ge c_{\rm in}(q,r)\varrho(B_r(\theta^\star)).
    \label{eq:J_inside_mass_lower}
\end{equation}

Second, take $\theta\notin N_{r_G}(\Theta)$. Then $\dist(\theta,\Theta)>r_G$. We claim that
\begin{equation}
    L(\theta)-L^\star
    >\min\left\{L_\infty,(\eta_Lr_G)^{1/\nu_L}\right\}.
    \label{eq:L_outside_case_split_result}
\end{equation}
Indeed, if $L(\theta)-L^\star>L_\infty$, then \eqref{eq:L_outside_case_split_result} is immediate. If $L(\theta)-L^\star\le L_\infty$, then \eqref{eq:L_error_bound} applies. If $L(\theta)-L^\star\le (\eta_Lr_G)^{1/\nu_L}$, then
\begin{equation}
    \dist(\theta,\Theta)
    \le \eta_L^{-1}\big(L(\theta)-L^\star\big)^{\nu_L}
    \le \eta_L^{-1}\eta_Lr_G=r_G,
\end{equation}
contradicting $\theta\notin N_{r_G}(\Theta)$. Hence \eqref{eq:L_outside_case_split_result} holds.
Combining \eqref{eq:L_outside_case_split_result} with \eqref{eq:laplace_q_condition} gives
\begin{equation}
    q-L(\theta)\le -\delta_q,
    \qquad \theta\in N_{r_G}(\Theta)^c.
\end{equation}
Since $s$ is increasing,
\begin{equation}
    \eta(\theta)
    \le s\left(-\frac{\delta_q}{\tau}\right)
    =c_{\rm out}(\delta_q),
    \qquad \theta\in N_{r_G}(\Theta)^c.
    \label{eq:eta_outside_upper}
\end{equation}

Let
\begin{equation}
    Z:=\int_{\R^d}e^{-\alpha G(\theta)}\dd J(\theta).
\end{equation}
By \eqref{eq:J_inside_mass_lower},
\begin{equation}
    Z
    \ge \int_{B_r(\theta^\star)}e^{-\alpha G(\theta)}\dd J(\theta)
    \ge e^{-\alpha\sup_{B_r(\theta^\star)}G}
    c_{\rm in}(q,r)\varrho(B_r(\theta^\star)).
    \label{eq:Z_inside_lower}
\end{equation}
Since $\tilde\theta\in B_{r_G}(\theta^\star)$,
\begin{equation}
    \norm{m-\theta^\star}_2
    \le r_G+\norm{m-\tilde\theta}_2.
    \label{eq:m_theta_triangle}
\end{equation}
Define
\begin{equation}
    \tilde r:=\eta_G^{-1}(u+\widetilde G_r)^{\nu_G}.
\end{equation}
Then
\begin{equation}
    \norm{m-\tilde\theta}_2
    \le T_1+T_2+T_3,
\end{equation}
where
\begin{align}
    T_1&:=Z^{-1}\int_{B_{\tilde r}(\tilde\theta)}\norm{\theta-\tilde\theta}_2e^{-\alpha G(\theta)}\dd J(\theta),                                      \\
    T_2&:=Z^{-1}\int_{N_{r_G}(\Theta)\setminus B_{\tilde r}(\tilde\theta)}\norm{\theta-\tilde\theta}_2e^{-\alpha G(\theta)}\dd J(\theta),                  \\
    T_3&:=Z^{-1}\int_{N_{r_G}(\Theta)^c}\norm{\theta-\tilde\theta}_2e^{-\alpha G(\theta)}\dd J(\theta).
\end{align}
The first term satisfies $T_1\le\tilde r$ because $Z$ is the full normalizing denominator.

For $T_2$, take $\theta\in N_{r_G}(\Theta)\setminus B_{\tilde r}(\tilde\theta)$. If $G(\theta)-G(\tilde\theta)\le u+\widetilde G_r$, then $G(\theta)-G(\tilde\theta)\le G_\infty$ by \eqref{eq:laplace_other_conditions}; applying \eqref{eq:G_error_bound} gives
\begin{equation}
    \norm{\theta-\tilde\theta}_2
    \le \eta_G^{-1}\big(G(\theta)-G(\tilde\theta)\big)^{\nu_G}
    \le \eta_G^{-1}(u+\widetilde G_r)^{\nu_G}=\tilde r,
\end{equation}
contradicting $\theta\notin B_{\tilde r}(\tilde\theta)$. Therefore
\begin{equation}
    G(\theta)-G(\tilde\theta)>u+\widetilde G_r.
    \label{eq:G_gap_T2}
\end{equation}
For every $\xi\in B_r(\theta^\star)$, by definition of $\widetilde G_r$,
\begin{equation}
    G(\xi)-G(\tilde\theta)\le\widetilde G_r.
\end{equation}
Combining this with \eqref{eq:G_gap_T2} gives $G(\theta)-G(\xi)>u$, hence
\begin{equation}
    e^{-\alpha G(\theta)}\le e^{-\alpha u}e^{-\alpha G(\xi)},
    \qquad \xi\in B_r(\theta^\star).
\end{equation}
Integrating this inequality with respect to $J(\dd\xi)$ over $B_r(\theta^\star)$ yields
\begin{equation}
    e^{-\alpha G(\theta)}J(B_r(\theta^\star))
    \le e^{-\alpha u}\int_{B_r(\theta^\star)}e^{-\alpha G(\xi)}\dd J(\xi)
    \le e^{-\alpha u}Z.
\end{equation}
Using \eqref{eq:J_inside_mass_lower},
\begin{equation}
    e^{-\alpha G(\theta)}
    \le \frac{e^{-\alpha u}Z}{c_{\rm in}(q,r)\varrho(B_r(\theta^\star))}.
\end{equation}
Consequently,
\begin{equation}
    T_2
    \le \frac{e^{-\alpha u}}{c_{\rm in}(q,r)\varrho(B_r(\theta^\star))}
    \int_{\R^d}\norm{\theta-\tilde\theta}_2\dd J(\theta).
    \label{eq:T2_bound}
\end{equation}

For $T_3$, use \eqref{eq:eta_outside_upper}, $G\ge G_{\min}$, and \eqref{eq:Z_inside_lower}:
\begin{align}
    T_3
    &\le Z^{-1}e^{-\alpha G_{\min}}c_{\rm out}(\delta_q)
    \int_{\R^d}\norm{\theta-\tilde\theta}_2\varrho(\dd\theta)                              \\
    &\le
    \frac{e^{\alpha(\sup_{B_r(\theta^\star)}G-G_{\min})}c_{\rm out}(\delta_q)}{c_{\rm in}(q,r)\varrho(B_r(\theta^\star))}
    \int_{\R^d}\norm{\theta-\tilde\theta}_2\varrho(\dd\theta)                              \\
    &=\frac{e^{\alpha\Delta_r}c_{\rm out}(\delta_q)}{c_{\rm in}(q,r)\varrho(B_r(\theta^\star))}
    \int_{\R^d}\norm{\theta-\tilde\theta}_2\varrho(\dd\theta).
    \label{eq:T3_bound}
\end{align}
Combining \eqref{eq:m_theta_triangle}, the bounds on $T_1$, \eqref{eq:T2_bound}, and \eqref{eq:T3_bound} proves \eqref{eq:laplace_first_bound}.

It remains to prove \eqref{eq:laplace_V_bound}. Since $0<\eta<1$ and $J(\R^d)=\beta$,
\begin{align}
    \int_{\R^d}\norm{\theta-\tilde\theta_G}_2\dd J(\theta)
    &\le \int_{\R^d}\norm{\theta-\theta^\star}_2\dd J(\theta)+r_GJ(\R^d)                  \\
    &\le \int_{\R^d}\norm{\theta-\theta^\star}_2\varrho(\dd\theta)+\beta r_G              \\
    &\le \sqrt{2V_\varrho}+\beta r_G,
\end{align}
where the last step is Cauchy's inequality. Similarly,
\begin{equation}
    \int_{\R^d}\norm{\theta-\tilde\theta_G}_2\varrho(\dd\theta)
    \le \sqrt{2V_\varrho}+r_G.
\end{equation}
Substituting these two estimates into \eqref{eq:laplace_first_bound} gives \eqref{eq:laplace_V_bound}.
\end{proof}

\section{Lower bound on the mass near the target}

\begin{proposition}[Lower bound on $\rho_{t,\tau}(B_r(\theta^\star))$]\label{prop:mass_lower_bound}
Let $T>0$ and $r>0$. Assume that $\rho_{t,\tau}$ solves the Fokker--Planck equation associated with \eqref{eq:mf_sde} and that
\begin{equation}
    \sup_{t\in[0,T]}\int_{\R^d}\norm{x}_2^4\rho_{t,\tau}(\dd x)
    \le C_{\rm mf,4}.
    \label{eq:mf_fourth_assumption}
\end{equation}
Define
\begin{equation}
    B_0:=C_mC_{\rm mf,4}^{1/4}+\norm{\theta^\star}_2.
    \label{eq:B0_def}
\end{equation}
Let
\begin{equation}
    \phi_r(\theta):=
    \begin{cases}
        \displaystyle \exp\left(1-\frac{r^2}{r^2-\norm{\theta-\theta^\star}_2^2}\right),
        &\norm{\theta-\theta^\star}_2<r,\\[1ex]
        0,&\norm{\theta-\theta^\star}_2\ge r.
    \end{cases}
    \label{eq:bump_def}
\end{equation}
Choose $c\in(1/2,1)$ satisfying
\begin{equation}
    d(1-c)^2\le c(2c-1).
    \label{eq:c_condition}
\end{equation}
Define
\begin{equation}
    K_1:=\frac{2\lambda(cr+B_0\sqrt c)}{(1-c)^2r}
    +\frac{2\sigma^2(cr^2+B_0^2)(2c+d)}{(1-c)^4r^2},
    \qquad
    K_2:=\frac{\lambda^2}{\sigma^2c(2c-1)},
    \label{eq:K1K2_def}
\end{equation}
\begin{equation}
    p:=2\max\{K_1,K_2\}.
    \label{eq:p_def}
\end{equation}
Then, for every $t\in[0,T]$,
\begin{equation}
    \rho_{t,\tau}(B_r(\theta^\star))
    \ge \left(\int_{\R^d}\phi_r(\theta)\rho_0(\dd\theta)\right)e^{-pt}.
    \label{eq:mass_lower_final}
\end{equation}
\end{proposition}

\begin{proof}
Since $0\le\phi_r\le1$ and $\supp(\phi_r)=B_r(\theta^\star)$,
\begin{equation}
    \rho_{t,\tau}(B_r(\theta^\star))
    \ge \int_{\R^d}\phi_r(\theta)\rho_{t,\tau}(\dd\theta).
    \label{eq:mass_phi_relation}
\end{equation}
By the consensus-moment stability bound \eqref{eq:consensus_moment_stability} and \eqref{eq:mf_fourth_assumption},
\begin{equation}
    \norm{m(\rho_{t,\tau})-\theta^\star}_2
    \le C_mC_{\rm mf,4}^{1/4}+\norm{\theta^\star}_2
    =B_0.
    \label{eq:m_minus_star_B0}
\end{equation}
Set
\begin{equation}
    y:=\theta-\theta^\star,
    \qquad
    s_\theta:=\norm{y}_2^2,
    \qquad
    h:=r^2-s_\theta,
    \qquad
    m_t:=m(\rho_{t,\tau}),
    \qquad
    w_t:=m_t-\theta^\star.
\end{equation}
Inside $B_r(\theta^\star)$, direct differentiation gives
\begin{equation}
    \nabla\phi_r(\theta)
    =-\frac{2r^2y}{h^2}\phi_r(\theta),
    \label{eq:bump_grad}
\end{equation}
\begin{equation}
    \Delta\phi_r(\theta)
    =\frac{2r^2}{h^4}\left(2(2s_\theta-r^2)s_\theta-dh^2\right)\phi_r(\theta).
    \label{eq:bump_laplacian}
\end{equation}
Outside $B_r(\theta^\star)$ the function and its first two derivatives vanish. The weak formulation gives
\begin{equation}
    \frac{\dd}{\dd t}\int\phi_r\dd\rho_{t,\tau}
    =\int_{\R^d}\big(T_1(\theta,t)+T_2(\theta,t)\big)\rho_{t,\tau}(\dd\theta),
    \label{eq:phi_derivative}
\end{equation}
where, using \eqref{eq:D_identities},
\begin{equation}
    T_1:=-\lambda\ip{\theta-m_t}{\nabla\phi_r(\theta)},
    \qquad
    T_2:=\frac{\sigma^2}{2}\norm{\theta-m_t}_2^2\Delta\phi_r(\theta).
\end{equation}
We prove pointwise that
\begin{equation}
    T_1(\theta,t)+T_2(\theta,t)\ge -p\phi_r(\theta).
    \label{eq:pointwise_mass_bound}
\end{equation}
The claim is trivial outside $B_r(\theta^\star)$. Inside the ball, write
\begin{equation}
    z:=\theta-m_t=y-w_t.
\end{equation}

\emph{Case 1: $s_\theta\le cr^2$.} Then $h\ge(1-c)r^2$ and $\norm{y}_2\le\sqrt c\,r$. By \eqref{eq:bump_grad},
\begin{align}
    T_1
    &=\frac{2\lambda r^2}{h^2}\ip{z}{y}\phi_r
    \ge -\frac{2\lambda r^2}{h^2}\left(\norm{y}_2^2+\norm{w_t}_2\norm{y}_2\right)\phi_r       \\
    &\ge -\frac{2\lambda r^2}{(1-c)^2r^4}\left(cr^2+B_0\sqrt c\,r\right)\phi_r
    =-\frac{2\lambda(cr+B_0\sqrt c)}{(1-c)^2r}\phi_r.
    \label{eq:T1_case1}
\end{align}
Also,
\begin{equation}
    \norm{z}_2^2\le2(\norm{y}_2^2+\norm{w_t}_2^2)\le2(cr^2+B_0^2).
    \label{eq:z_case1}
\end{equation}
Since $s_\theta\le cr^2$ and $h\le r^2$,
\begin{equation}
    2(2s_\theta-r^2)s_\theta-dh^2
    \ge -(2c+d)r^4.
    \label{eq:bracket_case1}
\end{equation}
Using \eqref{eq:bump_laplacian}, \eqref{eq:z_case1}, \eqref{eq:bracket_case1}, and $h\ge(1-c)r^2$ gives
\begin{equation}
    T_2
    \ge -\frac{2\sigma^2(cr^2+B_0^2)(2c+d)}{(1-c)^4r^2}\phi_r.
    \label{eq:T2_case1}
\end{equation}
Equations \eqref{eq:T1_case1} and \eqref{eq:T2_case1} imply $T_1+T_2\ge -K_1\phi_r\ge-p\phi_r$.

\emph{Case 2: $cr^2<s_\theta<r^2$.} Since $s_\theta>cr^2$ and $h^2\le(1-c)^2r^4$,
\begin{align}
    2(2s_\theta-r^2)s_\theta-dh^2
    &\ge 2(2c-1)cr^4-d(1-c)^2r^4                                               \\
    &\ge c(2c-1)r^4,
    \label{eq:bracket_case2}
\end{align}
where the last inequality uses \eqref{eq:c_condition}. Hence
\begin{equation}
    T_2
    \ge \frac{\sigma^2r^2}{h^4}c(2c-1)r^4\norm{z}_2^2\phi_r.
    \label{eq:T2_case2}
\end{equation}
Moreover,
\begin{equation}
    T_1
    =\frac{2\lambda r^2}{h^2}\ip{z}{y}\phi_r
    \ge -\frac{2\lambda r^2}{h^2}\norm{z}_2\norm{y}_2\phi_r.
    \label{eq:T1_case2}
\end{equation}
For $X:=\norm{z}_2$, the expression $aX^2-bX$ is bounded below by $-b^2/(4a)$ with
\begin{equation}
    a:=\frac{\sigma^2r^2c(2c-1)r^4}{h^4},
    \qquad
    b:=\frac{2\lambda r^2\norm{y}_2}{h^2}.
\end{equation}
Combining \eqref{eq:T2_case2} and \eqref{eq:T1_case2} therefore yields
\begin{equation}
    T_1+T_2
    \ge -\frac{\lambda^2\norm{y}_2^2}{\sigma^2c(2c-1)r^2}\phi_r
    \ge -\frac{\lambda^2}{\sigma^2c(2c-1)}\phi_r
    =-K_2\phi_r
    \ge -p\phi_r.
\end{equation}
Thus \eqref{eq:pointwise_mass_bound} holds in all cases.

Substituting \eqref{eq:pointwise_mass_bound} into \eqref{eq:phi_derivative} gives
\begin{equation}
    \frac{\dd}{\dd t}\int\phi_r\dd\rho_{t,\tau}
    \ge -p\int\phi_r\dd\rho_{t,\tau}.
\end{equation}
Gronwall's inequality gives
\begin{equation}
    \int\phi_r\dd\rho_{t,\tau}
    \ge \left(\int\phi_r\dd\rho_0\right)e^{-pt}.
\end{equation}
Combining this with \eqref{eq:mass_phi_relation} proves \eqref{eq:mass_lower_final}.
\end{proof}

\section{Mean-field approximation on the cutoff event}

Throughout this section, fix $T,M>0$, and suppose Assumption~\ref{ass:quantile_monotonicity} holds for the family $\mathfrak M^N_{T,M}$ in \eqref{eq:measure_family_quantile}. Define
\begin{equation}
    \kappa>0,
    \qquad
    C_q:=\frac{L_sL_L}{\tau\kappa}.
    \label{eq:Cq_def}
\end{equation}
Set
\begin{equation}
    b_M:=b(M),
    \qquad
    b_{\rm mf}:=b(C_{\rm bd}(T)),
    \qquad
    b_{M,T}:=\min\{b_M,b_{\rm mf}\},
    \label{eq:bMT_def}
\end{equation}
\begin{equation}
    a_M:=a(M),
    \qquad
    a_{\rm mf}:=a(C_{\rm bd}(T)),
    \qquad
    a_{M,T}:=\max\{a_M,a_{\rm mf}\}.
    \label{eq:aM_amf_def}
\end{equation}
Define
\begin{equation}
    C_{\phi,x}:=e^{-\alpha G_{\min}}\left(1+\alpha L_GM^{1/4}+\frac{L_sL_L}{\tau}M^{1/4}\right),
    \qquad
    C_{\phi,q}:=e^{-\alpha G_{\min}}\frac{L_s}{\tau}M^{1/4},
    \label{eq:Cphix_Cphiq_def}
\end{equation}
\begin{equation}
    \widetilde C_\phi:=C_{\phi,x}+C_{\phi,q}C_q,
    \label{eq:Cphi_tilde_def}
\end{equation}
\begin{equation}
    C_{\psi,x}:=e^{-\alpha G_{\min}}\left(\alpha L_G+\frac{L_sL_L}{\tau}\right),
    \qquad
    C_{\psi,q}:=e^{-\alpha G_{\min}}\frac{L_s}{\tau},
    \label{eq:Cpsix_Cpsiq_def}
\end{equation}
\begin{equation}
    \widetilde C_\psi:=C_{\psi,x}+C_{\psi,q}C_q.
    \label{eq:Cpsi_tilde_def}
\end{equation}
Finally define
\begin{equation}
    C_{\rm coup}:=2b_{M,T}^{-2}\widetilde C_\phi^2
    +2a_{M,T}^2b_{M,T}^{-4}\widetilde C_\psi^2,
    \label{eq:Ccoup_def}
\end{equation}
\begin{equation}
    C_{q,{\rm emp}}:=\frac{1}{4\kappa^2},
    \label{eq:Cqemp_def}
\end{equation}
\begin{equation}
    C_{A,{\rm emp}}:=2C_{\phi,q}^2C_{q,{\rm emp}}+2e^{-2\alpha G_{\min}}C_{\rm bd}(T)^{1/2},
    \qquad
    C_{B,{\rm emp}}:=2C_{\psi,q}^2C_{q,{\rm emp}}+2e^{-2\alpha G_{\min}},
    \label{eq:CA_CB_emp_def}
\end{equation}
\begin{equation}
    C_{\rm emp}:=2b_{M,T}^{-2}C_{A,{\rm emp}}
    +2a_{M,T}^2b_{M,T}^{-4}C_{B,{\rm emp}}.
    \label{eq:Cemp_def}
\end{equation}
With
\begin{equation}
    C_0:=-\lambda+2\sigma^2d,
    \qquad
    C_1:=\lambda+2\sigma^2d,
    \qquad
    K_{\rm MFA}:=C_0+2C_1C_{\rm coup},
    \label{eq:C0C1KMFA_def}
\end{equation}
define
\begin{equation}
    C_{\rm MFA}:=4C_1C_{\rm emp}T\exp\big(\max\{K_{\rm MFA},0\}T\big).
    \label{eq:CMFA_def}
\end{equation}

\begin{lemma}[Second-moment bound for empirical averages]\label{lem:empirical_second_moment}
For
\begin{equation}
    \phi_q(x):=xe^{-\alpha G(x)}s\left(\frac{q-L(x)}{\tau}\right),
    \qquad
    \psi_q(x):=e^{-\alpha G(x)}s\left(\frac{q-L(x)}{\tau}\right),
\end{equation}
one has
\begin{equation}
    \sup_{t\in[0,T]}\E\left[\norm{\phi_{q_{\rho_{t,\tau}}}(\bar\Theta^1_{t,\tau})}_2^2
    +|\psi_{q_{\rho_{t,\tau}}}(\bar\Theta^1_{t,\tau})|^2\right]
    \le C_{\rm mom}(T),
\end{equation}
where
\begin{equation}
    C_{\rm mom}(T):=e^{-2\alpha G_{\min}}\big(C_{\rm bd}(T)^{1/2}+1\big).
\end{equation}
\end{lemma}

\begin{proof}
Since $0<s<1$ and $G\ge G_{\min}$,
\begin{equation}
    \norm{\phi_{q_{\rho_{t,\tau}}}(x)}_2^2
    \le e^{-2\alpha G_{\min}}\norm{x}_2^2,
    \qquad
    |\psi_{q_{\rho_{t,\tau}}}(x)|^2
    \le e^{-2\alpha G_{\min}}.
\end{equation}
Using
\begin{equation}
    \E\norm{\bar\Theta^1_{t,\tau}}_2^2
    \le \left(\E\norm{\bar\Theta^1_{t,\tau}}_2^4\right)^{1/2}
    \le C_{\rm bd}(T)^{1/2}
\end{equation}
proves the claim.
\end{proof}

\begin{proposition}[Mean-field approximation on $\Omega_M$]\label{prop:MFA}
Assume Assumption~\ref{ass:primitive}. Fix $T,M>0$ and suppose Assumption~\ref{ass:quantile_monotonicity} holds for the family $\mathfrak M^N_{T,M}$ in \eqref{eq:measure_family_quantile}. If
\begin{equation}
    \Prob(\Omega_M)\ge \frac12,
    \label{eq:Omega_M_half}
\end{equation}
then
\begin{equation}
    \max_{1\le i\le N}\sup_{t\in[0,T]}
    \E\left[\norm{\Theta^{i,N}_{t,\tau}-\bar\Theta^i_{t,\tau}}_2^2\mid\Omega_M\right]
    \le \frac{C_{\rm MFA}}{N},
    \label{eq:MFA_result}
\end{equation}
where $C_{\rm MFA}$ is given in \eqref{eq:CMFA_def}.
\end{proposition}

\begin{proof}
Set
\begin{equation}
    e^i_t:=\Theta^{i,N}_{t,\tau}-\bar\Theta^i_{t,\tau},
    \qquad
    q^{N,{\rm int}}_t:=q_{\rho^{N,{\rm int}}_{t,\tau}},
    \qquad
    \bar q^N_t:=q_{\bar\rho^N_{t,\tau}},
    \qquad
    q_t:=q_{\rho_{t,\tau}}.
\end{equation}
Apply Ito's formula to the stopped process $\norm{e^i_{t\wedge\tau_M}}_2^2$. After localizing the stochastic integral and using Lemma~\ref{lem:stopped_integral_ineq} with $Y_t=\norm{e^i_t}_2^2$, we obtain, in the distributional sense,
\begin{align}
    \frac{\dd}{\dd t}\E\left[\norm{e^i_t}_2^2I_M(t)\right]
    &\le 2\E\left[\ip{e^i_t}{-\lambda(e^i_t-(m(\rho^{N,{\rm int}}_{t,\tau})-m(\rho_{t,\tau})))}I_M(t)\right]       \\
    &\quad +\sigma^2\E\left[\norm{D(\Theta^{i,N}_{t,\tau}-m(\rho^{N,{\rm int}}_{t,\tau}))
    -D(\bar\Theta^i_{t,\tau}-m(\rho_{t,\tau}))}_F^2I_M(t)\right].
    \label{eq:MFA_ito_start}
\end{align}
Indeed, before the stopping time $\tau_M$ this is the usual Ito identity for $\norm{e^i_t}_2^2$, and Lemma~\ref{lem:stopped_integral_ineq} converts the stopped identity into the displayed inequality for the indicator-weighted expectation.
Using $2\ip{x}{y}\le\norm{x}_2^2+\norm{y}_2^2$ and \eqref{eq:D_identities},
\begin{equation}
    \frac{\dd}{\dd t}\E\left[\norm{e^i_t}_2^2I_M(t)\right]
    \le C_0\E\left[\norm{e^i_t}_2^2I_M(t)\right]
    +C_1\E\left[\norm{m(\rho^{N,{\rm int}}_{t,\tau})-m(\rho_{t,\tau})}_2^2I_M(t)\right].
    \label{eq:MFA_diff_ineq_pre}
\end{equation}

\emph{Step 1: quantile difference between the two empirical measures.}
On $\{I_M(t)=1\}$, one has $\rho^{N,{\rm int}}_{t,\tau}=\rho^{N,{\rm int}}_{t\wedge\tau_M,\tau}$, so this interacting empirical measure belongs to $\mathfrak M^N_{T,M}$. Assumption~\ref{ass:quantile_monotonicity} and Lemma~\ref{lem:inverse_stability} applied with $\mu=\rho^{N,{\rm int}}_{t,\tau}$ and $\nu=\bar\rho^N_{t,\tau}$ give
\begin{equation}
    |q^{N,{\rm int}}_t-\bar q^N_t|I_M(t)
    \le \kappa^{-1}|F_{\rho^{N,{\rm int}}_{t,\tau}}(\bar q^N_t)-F_{\bar\rho^N_{t,\tau}}(\bar q^N_t)|I_M(t).
\end{equation}
Since $s$ and $L$ are Lipschitz,
\begin{align}
    |F_{\rho^{N,{\rm int}}_{t,\tau}}(\bar q^N_t)-F_{\bar\rho^N_{t,\tau}}(\bar q^N_t)|
    &\le \frac{L_s}{\tau}\frac1N\sum_{j=1}^N
    |L(\Theta^{j,N}_{t,\tau})-L(\bar\Theta^j_{t,\tau})|                         \\
    &\le \frac{L_sL_L}{\tau}\frac1N\sum_{j=1}^N\norm{e^j_t}_2.
\end{align}
Therefore, by Cauchy's inequality,
\begin{equation}
    |q^{N,{\rm int}}_t-\bar q^N_t|^2I_M(t)
    \le C_q^2\frac1N\sum_{j=1}^N\norm{e^j_t}_2^2I_M(t).
    \label{eq:emp_quantile_diff_bound}
\end{equation}

\emph{Step 2: consensus difference between the two empirical measures.}
For arbitrary $x,y\in\R^d$ and $q_1,q_2\in\R$,
\begin{align}
    \norm{\phi_{q_1}(x)-\phi_{q_2}(y)}_2
    &\le e^{-\alpha G_{\min}}\norm{x-y}_2
    +\alpha e^{-\alpha G_{\min}}L_G\norm{y}_2\norm{x-y}_2                                      \\
    &\quad +e^{-\alpha G_{\min}}\norm{x}_2\frac{L_s}{\tau}
    \big(|q_1-q_2|+L_L\norm{x-y}_2\big).
    \label{eq:phi_lipschitz_pointwise}
\end{align}
Indeed, this follows from
\begin{equation}
    \norm{xe^{-\alpha G(x)}-ye^{-\alpha G(y)}}_2
    \le e^{-\alpha G_{\min}}\norm{x-y}_2
    +\alpha e^{-\alpha G_{\min}}L_G\norm{y}_2\norm{x-y}_2
\end{equation}
and the Lipschitz property of $s$.
On $\{I_M(t)=1\}$, the cutoff gives
\begin{equation}
    \frac1N\sum_{j=1}^N\norm{\Theta^{j,N}_{t,\tau}}_2\le M^{1/4},
    \qquad
    \frac1N\sum_{j=1}^N\norm{\bar\Theta^j_{t,\tau}}_2\norm{e^j_t}_2
    \le M^{1/4}\left(\frac1N\sum_{j=1}^N\norm{e^j_t}_2^2\right)^{1/2}.
    \label{eq:cutoff_average_bounds}
\end{equation}
Averaging \eqref{eq:phi_lipschitz_pointwise}, using \eqref{eq:emp_quantile_diff_bound}, and then squaring gives
\begin{equation}
    \norm{A(\rho^{N,{\rm int}}_{t,\tau})-A(\bar\rho^N_{t,\tau})}_2^2I_M(t)
    \le \widetilde C_\phi^2\frac1N\sum_{j=1}^N\norm{e^j_t}_2^2I_M(t).
    \label{eq:A_emp_emp_bound}
\end{equation}
Similarly,
\begin{equation}
    |\psi_{q_1}(x)-\psi_{q_2}(y)|
    \le e^{-\alpha G_{\min}}\left(\alpha L_G+\frac{L_sL_L}{\tau}\right)\norm{x-y}_2
    +e^{-\alpha G_{\min}}\frac{L_s}{\tau}|q_1-q_2|,
\end{equation}
which yields
\begin{equation}
    |B(\rho^{N,{\rm int}}_{t,\tau})-B(\bar\rho^N_{t,\tau})|^2I_M(t)
    \le \widetilde C_\psi^2\frac1N\sum_{j=1}^N\norm{e^j_t}_2^2I_M(t).
    \label{eq:B_emp_emp_bound}
\end{equation}
On $\{I_M(t)=1\}$,
\begin{equation}
    \norm{A(\bar\rho^N_{t,\tau})}_2
    \le e^{-\alpha G_{\min}}
    \left(\int\norm{x}_2^2\dd J^L_{\beta,\tau}[\bar\rho^N_{t,\tau}](x)\right)^{1/2}\beta^{1/2}
    \le a_M.
    \label{eq:A_bar_aM}
\end{equation}
The quotient identity
\begin{equation}
    m(\rho)-m(\nu)
    =\frac{A(\rho)-A(\nu)}{B(\rho)}
    +A(\nu)\frac{B(\nu)-B(\rho)}{B(\rho)B(\nu)}
    \label{eq:quotient_identity}
\end{equation}
combined with the denominator bound $B\ge b_{M,T}$ from Lemma~\ref{lem:moment_denominator_bound}, \eqref{eq:A_emp_emp_bound}, \eqref{eq:B_emp_emp_bound}, \eqref{eq:A_bar_aM}, and $(a+b)^2\le2(a^2+b^2)$ gives
\begin{equation}
    \norm{m(\rho^{N,{\rm int}}_{t,\tau})-m(\bar\rho^N_{t,\tau})}_2^2I_M(t)
    \le C_{\rm coup}\frac1N\sum_{j=1}^N\norm{e^j_t}_2^2I_M(t).
    \label{eq:m_emp_emp_bound}
\end{equation}

\emph{Step 3: empirical fluctuation of the mean-field sample.}
On $\{I_M(t)=1\}$, Lemma~\ref{lem:inverse_stability} applied with $\mu=\bar\rho^N_{t,\tau}$ and $\nu=\rho_{t,\tau}$ gives
\begin{equation}
    |\bar q^N_t-q_t|I_M(t)
    \le \kappa^{-1}|F^N_t(q_t)-F_t(q_t)|I_M(t),
\end{equation}
where
\begin{equation}
    F^N_t(q):=\frac1N\sum_{j=1}^Ns\left(\frac{q-L(\bar\Theta^j_{t,\tau})}{\tau}\right)-\beta,
    \qquad
    F_t(q):=\int s\left(\frac{q-L(x)}{\tau}\right)\rho_{t,\tau}(\dd x)-\beta.
\end{equation}
The random variables
\begin{equation}
    Z_j:=s\left(\frac{q_t-L(\bar\Theta^j_{t,\tau})}{\tau}\right)
\end{equation}
are i.i.d., lie in $[0,1]$, and have mean $\beta$. Hence $\operatorname{Var}(Z_j)\le1/4$ and
\begin{align}
    \E\left[|\bar q^N_t-q_t|^2I_M(t)\right]
    &\le \kappa^{-2}\E\left[|F^N_t(q_t)-F_t(q_t)|^2I_M(t)\right] \\
    &\le \kappa^{-2}\E\left[|F^N_t(q_t)-F_t(q_t)|^2\right]
    \le \frac{1}{4\kappa^2N}
    =\frac{C_{q,{\rm emp}}}{N}.
    \label{eq:qbar_q_var_bound}
\end{align}
Next,
\begin{align}
    A(\bar\rho^N_{t,\tau})-A(\rho_{t,\tau})
    &=\frac1N\sum_{j=1}^N\big(\phi_{\bar q^N_t}(\bar\Theta^j_{t,\tau})-\phi_{q_t}(\bar\Theta^j_{t,\tau})\big)       \\
    &\quad +\left(\frac1N\sum_{j=1}^N\phi_{q_t}(\bar\Theta^j_{t,\tau})-\E\phi_{q_t}(\bar\Theta^1_{t,\tau})\right).
    \label{eq:A_bar_decomp}
\end{align}
The first term in \eqref{eq:A_bar_decomp} has norm at most $C_{\phi,q}|\bar q^N_t-q_t|$ on $\{I_M(t)=1\}$. The second term has second moment bounded by
\begin{equation}
    \frac1N\E\norm{\phi_{q_t}(\bar\Theta^1_{t,\tau})}_2^2
    \le \frac{e^{-2\alpha G_{\min}}C_{\rm bd}(T)^{1/2}}{N}
\end{equation}
by Lemma~\ref{lem:empirical_second_moment}. Using $(a+b)^2\le2(a^2+b^2)$ and \eqref{eq:qbar_q_var_bound},
\begin{equation}
    \E\left[\norm{A(\bar\rho^N_{t,\tau})-A(\rho_{t,\tau})}_2^2I_M(t)\right]
    \le \frac{C_{A,{\rm emp}}}{N}.
    \label{eq:A_emp_law_bound}
\end{equation}
The same argument for $B$ gives
\begin{equation}
    \E\left[|B(\bar\rho^N_{t,\tau})-B(\rho_{t,\tau})|^2I_M(t)\right]
    \le \frac{C_{B,{\rm emp}}}{N}.
    \label{eq:B_emp_law_bound}
\end{equation}
Furthermore,
\begin{equation}
    \norm{A(\rho_{t,\tau})}_2
    \le e^{-\alpha G_{\min}}\left(\int\norm{x}_2^2\,\dd J^L_{\beta,\tau}[\rho_{t,\tau}](x)\right)^{1/2}\beta^{1/2}
    \le \beta^{1/2}e^{-\alpha G_{\min}}C_{\rm bd}(T)^{1/4}=a_{\rm mf}.
    \label{eq:A_law_amf}
\end{equation}
Using \eqref{eq:quotient_identity}, the denominator bound $B\ge b_{M,T}$ from Lemma~\ref{lem:moment_denominator_bound}, \eqref{eq:A_emp_law_bound}, \eqref{eq:B_emp_law_bound}, \eqref{eq:A_law_amf}, and $(a+b)^2\le2(a^2+b^2)$,
\begin{equation}
    \E\left[\norm{m(\bar\rho^N_{t,\tau})-m(\rho_{t,\tau})}_2^2I_M(t)\right]
    \le \frac{C_{\rm emp}}{N}.
    \label{eq:m_emp_law_bound}
\end{equation}

\emph{Step 4: Gronwall closure.}
By
\begin{equation}
    m(\rho^{N,{\rm int}}_{t,\tau})-m(\rho_{t,\tau})
    =\big(m(\rho^{N,{\rm int}}_{t,\tau})-m(\bar\rho^N_{t,\tau})\big)
    +\big(m(\bar\rho^N_{t,\tau})-m(\rho_{t,\tau})\big),
\end{equation}
\eqref{eq:m_emp_emp_bound}, \eqref{eq:m_emp_law_bound}, and $(a+b)^2\le2(a^2+b^2)$ imply
\begin{equation}
    \E\left[\norm{m(\rho^{N,{\rm int}}_{t,\tau})-m(\rho_{t,\tau})}_2^2I_M(t)\right]
    \le 2C_{\rm coup}\frac1N\sum_{j=1}^N\E\left[\norm{e^j_t}_2^2I_M(t)\right]
    +\frac{2C_{\rm emp}}{N}.
    \label{eq:m_total_bound}
\end{equation}
Averaging \eqref{eq:MFA_diff_ineq_pre} over $i$ and setting
\begin{equation}
    E_t:=\frac1N\sum_{i=1}^N\E\left[\norm{e^i_t}_2^2I_M(t)\right]
\end{equation}
gives
\begin{equation}
    \dot E_t\le K_{\rm MFA}E_t+\frac{2C_1C_{\rm emp}}{N},
    \qquad
    E_0=0.
\end{equation}
Therefore
\begin{equation}
    E_t\le \frac{2C_1C_{\rm emp}T\exp(\max\{K_{\rm MFA},0\}T)}{N},
    \qquad t\in[0,T].
    \label{eq:Et_final}
\end{equation}
By exchangeability, the same upper bound holds for each $\E[\norm{e^i_t}_2^2I_M(t)]$. Since $I_M(T)\le I_M(t)$ and $\Prob(\Omega_M)\ge1/2$,
\begin{align}
    \E\left[\norm{e^i_t}_2^2\mid\Omega_M\right]
    &=\frac{\E\left[\norm{e^i_t}_2^2I_M(T)\right]}{\Prob(\Omega_M)}                    \\
    &\le 2\E\left[\norm{e^i_t}_2^2I_M(t)\right]                                           \\
    &\le \frac{4C_1C_{\rm emp}T\exp(\max\{K_{\rm MFA},0\}T)}{N}
    =\frac{C_{\rm MFA}}{N}.
\end{align}
This proves \eqref{eq:MFA_result}.
\end{proof}

\section{Direct mean-field convergence}

Define
\begin{equation}
    V_\tau(t):=\frac12\int_{\R^d}\norm{\theta-\theta^\star}_2^2\rho_{t,\tau}(\dd\theta),
    \qquad
    M_\tau(t):=\norm{m(\rho_{t,\tau})-\theta^\star}_2.
    \label{eq:V_M_def}
\end{equation}

\begin{lemma}[Lyapunov differential inequalities]\label{lem:lyapunov_ineq}
For almost every $t$,
\begin{equation}
    -aV_\tau(t)-b\sqrt{V_\tau(t)}M_\tau(t)
    \le \dot V_\tau(t)
    \le -aV_\tau(t)+b\sqrt{V_\tau(t)}M_\tau(t)+c_dM_\tau(t)^2,
    \label{eq:lyapunov_ineq}
\end{equation}
where
\begin{equation}
    a:=2\lambda-d\sigma^2,
    \qquad
    b:=\sqrt2(\lambda+d\sigma^2),
    \qquad
    c_d:=\frac{d\sigma^2}{2}.
    \label{eq:a_b_cd_def}
\end{equation}
\end{lemma}

\begin{proof}
Use the test function $\varphi(\theta)=\frac12\norm{\theta-\theta^\star}_2^2$. Since $\nabla\varphi=\theta-\theta^\star$ and $\nabla^2\varphi=\Id$, the weak formulation and \eqref{eq:D_identities} give
\begin{equation}
    \dot V_\tau(t)
    =-\lambda\int\ip{\theta-\theta^\star}{\theta-m_t}\rho_{t,\tau}(\dd\theta)
    +\frac{d\sigma^2}{2}\int\norm{\theta-m_t}_2^2\rho_{t,\tau}(\dd\theta),
    \label{eq:Vdot_start}
\end{equation}
where $m_t=m(\rho_{t,\tau})$. Let $\bar\theta_t:=\int\theta\rho_{t,\tau}(\dd\theta)$. Expanding around $\theta^\star$,
\begin{equation}
    -\lambda\int\ip{\theta-\theta^\star}{\theta-m_t}\rho_{t,\tau}(\dd\theta)
    =-2\lambda V_\tau(t)+\lambda\ip{\bar\theta_t-\theta^\star}{m_t-\theta^\star}.
    \label{eq:drift_expand}
\end{equation}
Similarly,
\begin{equation}
    \frac{d\sigma^2}{2}\int\norm{\theta-m_t}_2^2\rho_{t,\tau}(\dd\theta)
    =d\sigma^2V_\tau(t)-d\sigma^2\ip{\bar\theta_t-\theta^\star}{m_t-\theta^\star}
    +\frac{d\sigma^2}{2}M_\tau(t)^2.
    \label{eq:diff_expand}
\end{equation}
Combining \eqref{eq:Vdot_start}, \eqref{eq:drift_expand}, and \eqref{eq:diff_expand},
\begin{equation}
    \dot V_\tau(t)
    =-aV_\tau(t)+(\lambda+d\sigma^2)\ip{\bar\theta_t-\theta^\star}{m_t-\theta^\star}+c_dM_\tau(t)^2.
    \label{eq:Vdot_combined}
\end{equation}
Finally,
\begin{equation}
    \norm{\bar\theta_t-\theta^\star}_2
    \le\left(\int\norm{\theta-\theta^\star}_2^2\rho_{t,\tau}(\dd\theta)\right)^{1/2}
    =\sqrt{2V_\tau(t)}.
\end{equation}
Using this bound in \eqref{eq:Vdot_combined} gives the upper inequality in \eqref{eq:lyapunov_ineq}. Dropping the nonnegative term $c_dM_\tau(t)^2$ gives the lower inequality.
\end{proof}

\begin{theorem}[Conditional direct mean-field convergence without compact support]\label{thm:direct_mf_convergence}
Assume Assumption~\ref{ass:primitive}. Let $\varepsilon\in(0,V_\tau(0))$ and $\vartheta\in(0,1)$, and assume
\begin{equation}
    a=2\lambda-d\sigma^2>0.
\end{equation}
Define
\begin{equation}
    T^\star:=\frac{1}{(1-\vartheta)a}\log\left(\frac{V_\tau(0)}{\varepsilon}\right).
    \label{eq:Tstar_def}
\end{equation}
Assume that there exist $r_G\in(0,R_G]$, $r\in(0,r_G]$, $u>0$, and $\delta_q>0$ such that
\begin{equation}
    \int\phi_r(\theta)\rho_0(\dd\theta)>0,
    \label{eq:initial_local_mass}
\end{equation}
\begin{equation}
    q_{\rho_{t,\tau}}+\delta_q
    \le L^\star+\min\left\{L_\infty,(\eta_Lr_G)^{1/\nu_L}\right\},
    \qquad t\in[0,T^\star],
    \label{eq:uniform_q_condition_mf}
\end{equation}
\begin{equation}
    u+\widetilde G_r\le G_\infty,
    \qquad
    c_{\rm in}:=\inf_{t\in[0,T^\star]}
    s\left(\frac{q_{\rho_{t,\tau}}-L^\star-L_Lr}{\tau}\right)>0,
    \label{eq:cin_direct_def}
\end{equation}
where
\begin{equation}
    \tilde\theta_G:=\tilde\theta_{r_G},
    \qquad
    \widetilde G_r:=\sup_{\theta\in B_r(\theta^\star)}\big(G(\theta)-G(\tilde\theta_G)\big),
    \qquad
    \Delta_r:=\sup_{\theta\in B_r(\theta^\star)}G(\theta)-G_{\min}.
\end{equation}
Set
\begin{equation}
    C_{\rm mf,4}:=C_{\rm bd}(T^\star).
    \label{eq:Cmf4_direct}
\end{equation}
Let $B_0$, $K_1$, $K_2$, and $p$ be defined by \eqref{eq:B0_def}, \eqref{eq:K1K2_def}, and \eqref{eq:p_def} with $T=T^\star$ and $C_{\rm mf,4}=C_{\rm bd}(T^\star)$. Define
\begin{equation}
    m_\star:=\left(\int\phi_r(\theta)\rho_0(\dd\theta)\right)e^{-pT^\star},
    \label{eq:mstar_def}
\end{equation}
\begin{equation}
    c_{\rm out}:=s\left(-\frac{\delta_q}{\tau}\right),
    \label{eq:cout_direct_def}
\end{equation}
\begin{equation}
    A_\star
    :=r_G+\frac{(u+\widetilde G_r)^{\nu_G}}{\eta_G}
    +\frac{\beta r_Ge^{-\alpha u}+r_Ge^{\alpha\Delta_r}c_{\rm out}}{c_{\rm in}m_\star},
    \label{eq:Astar_def}
\end{equation}
\begin{equation}
    B_\star
    :=\frac{\sqrt2\big(e^{-\alpha u}+e^{\alpha\Delta_r}c_{\rm out}\big)}{c_{\rm in}m_\star}.
    \label{eq:Bstar_def}
\end{equation}
Assume the two explicit smallness conditions
\begin{equation}
    bB_\star+c_dB_\star^2
    +\frac{b+2c_dB_\star}{\sqrt\varepsilon}A_\star
    +\frac{c_d}{\varepsilon}A_\star^2
    \le \vartheta a,
    \label{eq:smallness_upper}
\end{equation}
\begin{equation}
    bB_\star+\frac{b}{\sqrt\varepsilon}A_\star
    \le \frac{\vartheta a}{2}.
    \label{eq:smallness_lower}
\end{equation}
Then there exists
\begin{equation}
    T_\varepsilon\in\left[\frac{1-\vartheta}{1+\vartheta/2}T^\star,T^\star\right]
    \label{eq:T_epsilon_interval}
\end{equation}
such that $V_\tau(T_\varepsilon)=\varepsilon$, and for every $t\in[0,T_\varepsilon]$,
\begin{equation}
    W_2^2(\rho_{t,\tau},\delta_{\theta^\star})
    =2V_\tau(t)
    \le 2V_\tau(0)e^{-(1-\vartheta)(2\lambda-d\sigma^2)t}.
    \label{eq:direct_mf_final}
\end{equation}
\end{theorem}

\begin{proof}
By Lemma~\ref{lem:moment_bound}, condition \eqref{eq:mf_fourth_assumption} holds with $C_{\rm mf,4}=C_{\rm bd}(T^\star)$. Proposition~\ref{prop:mass_lower_bound} gives
\begin{equation}
    \rho_{t,\tau}(B_r(\theta^\star))\ge m_\star,
    \qquad t\in[0,T^\star].
    \label{eq:rho_mass_mstar}
\end{equation}
Combining \eqref{eq:rho_mass_mstar}, Proposition~\ref{prop:laplace_no_compact}, and the definitions of $c_{\rm in}$, $c_{\rm out}$, $A_\star$, and $B_\star$ yields
\begin{equation}
    M_\tau(t)\le A_\star+B_\star\sqrt{V_\tau(t)},
    \qquad t\in[0,T^\star].
    \label{eq:M_bound_A_B}
\end{equation}
Let
\begin{equation}
    T_\varepsilon:=\inf\{t\in[0,T^\star]:V_\tau(t)\le\varepsilon\}.
    \label{eq:hitting_time_def}
\end{equation}
For $t\le T_\varepsilon$, $V_\tau(t)\ge\varepsilon$. By the upper inequality in Lemma~\ref{lem:lyapunov_ineq} and \eqref{eq:M_bound_A_B},
\begin{align}
    \dot V_\tau(t)
    &\le -aV_\tau(t)+b\sqrt{V_\tau(t)}\big(A_\star+B_\star\sqrt{V_\tau(t)}\big)
    +c_d\big(A_\star+B_\star\sqrt{V_\tau(t)}\big)^2                                             \\
    &=-\big(a-bB_\star-c_dB_\star^2\big)V_\tau(t)
    +(b+2c_dB_\star)A_\star\sqrt{V_\tau(t)}+c_dA_\star^2.
\end{align}
Since $V_\tau(t)\ge\varepsilon$, we have $\sqrt{V_\tau(t)}\le V_\tau(t)/\sqrt\varepsilon$ and $1\le V_\tau(t)/\varepsilon$. Hence
\begin{equation}
    \dot V_\tau(t)
    \le -\left(a-bB_\star-c_dB_\star^2
    -\frac{b+2c_dB_\star}{\sqrt\varepsilon}A_\star
    -\frac{c_d}{\varepsilon}A_\star^2\right)V_\tau(t).
\end{equation}
By \eqref{eq:smallness_upper},
\begin{equation}
    \dot V_\tau(t)\le -(1-\vartheta)aV_\tau(t),
    \qquad t\le T_\varepsilon.
\end{equation}
Therefore
\begin{equation}
    V_\tau(t)\le V_\tau(0)e^{-(1-\vartheta)at},
    \qquad t\le T_\varepsilon.
\end{equation}
At $t=T^\star$, the right-hand side equals $\varepsilon$ by \eqref{eq:Tstar_def}; hence $T_\varepsilon\le T^\star$ and $V_\tau(T_\varepsilon)=\varepsilon$.

For the lower hitting-time bound, use the lower inequality in Lemma~\ref{lem:lyapunov_ineq} and \eqref{eq:M_bound_A_B}. For $t\le T_\varepsilon$,
\begin{align}
    \dot V_\tau(t)
    &\ge -aV_\tau(t)-b\sqrt{V_\tau(t)}\big(A_\star+B_\star\sqrt{V_\tau(t)}\big)      \\
    &\ge -\left(a+bB_\star+\frac{b}{\sqrt\varepsilon}A_\star\right)V_\tau(t).
\end{align}
By \eqref{eq:smallness_lower},
\begin{equation}
    \dot V_\tau(t)\ge -(1+\vartheta/2)aV_\tau(t).
\end{equation}
Thus
\begin{equation}
    V_\tau(t)\ge V_\tau(0)e^{-(1+\vartheta/2)at},
    \qquad t\le T_\varepsilon.
\end{equation}
Since $V_\tau(T_\varepsilon)=\varepsilon$, comparison with \eqref{eq:Tstar_def} gives
\begin{equation}
    T_\varepsilon
    \ge \frac{1-\vartheta}{1+\vartheta/2}T^\star.
\end{equation}
The Wasserstein estimate follows from
\begin{equation}
    W_2^2(\rho_{t,\tau},\delta_{\theta^\star})=2V_\tau(t).
\end{equation}
\end{proof}

\begin{remark}[No circular parameter choice]\label{rem:no_circularity}
The proof fixes $(\alpha,\beta,\tau,\lambda,\sigma,r,r_G,u,\delta_q)$ first. Then the constants are computed in the order
\begin{equation}
    C_m,C_{\rm bd}
    \longrightarrow B_0,p,m_\star
    \longrightarrow A_\star,B_\star
    \longrightarrow T_\varepsilon,C_{\rm MFA},\text{probability bound}.
\end{equation}
No later constant is used to define an earlier one. The smallness conditions \eqref{eq:smallness_upper}--\eqref{eq:smallness_lower} are final verifiable inequalities, not recursive prescriptions.
\end{remark}

\section{Direct numerical convergence}

Define the empirical averages
\begin{equation}
    \widehat\theta^N_{K,\tau}:=\frac1N\sum_{i=1}^N\theta^i_{K,\tau},
    \qquad
    \widehat\Theta^{N,{\rm int}}_{T,\tau}:=\frac1N\sum_{i=1}^N\Theta^{i,N}_{T,\tau},
    \qquad
    \widehat{\bar\Theta}^{N}_{T,\tau}:=\frac1N\sum_{i=1}^N\bar\Theta^i_{T,\tau}.
\end{equation}
Young's inequality gives
\begin{align}
    \norm{\widehat\theta^N_{K,\tau}-\theta^\star}_2^2
    &\le 3\norm{\widehat\theta^N_{K,\tau}-\widehat\Theta^{N,{\rm int}}_{T,\tau}}_2^2
    +3\norm{\widehat\Theta^{N,{\rm int}}_{T,\tau}-\widehat{\bar\Theta}^{N}_{T,\tau}}_2^2
    +3\norm{\widehat{\bar\Theta}^{N}_{T,\tau}-\theta^\star}_2^2.
    \label{eq:three_term_decomp}
\end{align}

\begin{theorem}[Numerical convergence in probability]\label{thm:numerical_convergence}
Assume Assumption~\ref{ass:primitive}. Let $T=T_\varepsilon$ be the hitting time supplied by Theorem~\ref{thm:direct_mf_convergence}, and let $K\Delta t=T$. Assume Assumption~\ref{ass:quantile_monotonicity} holds for the family $\mathfrak M^N_{T,M}$ in \eqref{eq:measure_family_quantile}. Let $\delta_M\in(0,1/2]$ and choose
\begin{equation}
    M:=\frac{C_{\rm bd}(T)}{\delta_M}.
    \label{eq:M_choice}
\end{equation}
Then $\Prob(\Omega_M)\ge1-\delta_M\ge1/2$. Assume the numerical scheme satisfies the strong error estimate
\begin{equation}
    \E\left[\frac1N\sum_{i=1}^N\norm{\theta^i_{K,\tau}-\Theta^{i,N}_{T,\tau}}_2^2\right]
    \le C_{\rm NA}(\Delta t)^{2m_{\rm num}},
    \label{eq:numerical_assumption}
\end{equation}
where $C_{\rm NA}$ is the scheme-dependent strong-error constant and $m_{\rm num}>0$ is the strong order. If the hypotheses of Theorem~\ref{thm:direct_mf_convergence} hold and $V_\tau(T)=\varepsilon$, then, for every $\varepsilon_{\rm tot}>0$,
\begin{equation}
    \Prob\left(\norm{\widehat\theta^N_{K,\tau}-\theta^\star}_2^2\le\varepsilon_{\rm tot}\right)
    \ge
    1-\delta_M
    -\frac{6C_{\rm NA}(\Delta t)^{2m_{\rm num}}+3C_{\rm MFA}N^{-1}+12\varepsilon}{\varepsilon_{\rm tot}}.
    \label{eq:numerical_probability_bound}
\end{equation}
\end{theorem}

\begin{proof}
By Lemma~\ref{lem:moment_bound} and \eqref{eq:M_choice},
\begin{equation}
    \Prob(\Omega_M^c)\le\delta_M.
\end{equation}
Thus
\begin{equation}
    \Prob(\Omega_M)
    \ge1-\delta_M
    \ge\frac12.
    \label{eq:Omega_prob_numerical}
\end{equation}
On $\Omega_M$, use \eqref{eq:three_term_decomp}. For the first term, Jensen's inequality and \eqref{eq:numerical_assumption} give
\begin{align}
    \E\left[\norm{\widehat\theta^N_{K,\tau}-\widehat\Theta^{N,{\rm int}}_{T,\tau}}_2^2\mid\Omega_M\right]
    &\le \frac1{\Prob(\Omega_M)}
    \E\left[\frac1N\sum_{i=1}^N\norm{\theta^i_{K,\tau}-\Theta^{i,N}_{T,\tau}}_2^2\right]       \\
    &\le 2C_{\rm NA}(\Delta t)^{2m_{\rm num}}.
    \label{eq:first_term_num}
\end{align}
For the second term, Proposition~\ref{prop:MFA} gives
\begin{align}
    \E\left[\norm{\widehat\Theta^{N,{\rm int}}_{T,\tau}-\widehat{\bar\Theta}^{N}_{T,\tau}}_2^2\mid\Omega_M\right]
    &\le \frac1N\sum_{i=1}^N
    \E\left[\norm{\Theta^{i,N}_{T,\tau}-\bar\Theta^i_{T,\tau}}_2^2\mid\Omega_M\right]     \\
    &\le \frac{C_{\rm MFA}}{N}.
    \label{eq:second_term_num}
\end{align}
For the third term, Jensen's inequality, \eqref{eq:Omega_prob_numerical}, and $V_\tau(T)=\varepsilon$ yield
\begin{align}
    \E\left[\norm{\widehat{\bar\Theta}^{N}_{T,\tau}-\theta^\star}_2^2\mid\Omega_M\right]
    &\le \frac1{\Prob(\Omega_M)}
    \E\left[\norm{\widehat{\bar\Theta}^{N}_{T,\tau}-\theta^\star}_2^2\right]                  \\
    &\le 2\cdot\frac1N\sum_{i=1}^N\E\norm{\bar\Theta^i_{T,\tau}-\theta^\star}_2^2              \\
    &=4V_\tau(T)=4\varepsilon.
    \label{eq:third_term_num}
\end{align}
Substituting \eqref{eq:first_term_num}, \eqref{eq:second_term_num}, and \eqref{eq:third_term_num} into \eqref{eq:three_term_decomp},
\begin{equation}
    \E\left[\norm{\widehat\theta^N_{K,\tau}-\theta^\star}_2^2\mid\Omega_M\right]
    \le 6C_{\rm NA}(\Delta t)^{2m_{\rm num}}+3C_{\rm MFA}N^{-1}+12\varepsilon.
    \label{eq:conditional_error_total}
\end{equation}
Markov's inequality gives
\begin{align}
    \Prob\left(\norm{\widehat\theta^N_{K,\tau}-\theta^\star}_2^2>\varepsilon_{\rm tot}\right)
    &\le \Prob(\Omega_M^c)
    +\Prob\left(\norm{\widehat\theta^N_{K,\tau}-\theta^\star}_2^2>\varepsilon_{\rm tot}\mid\Omega_M\right)    \\
    &\le \delta_M
    +\frac{6C_{\rm NA}(\Delta t)^{2m_{\rm num}}+3C_{\rm MFA}N^{-1}+12\varepsilon}{\varepsilon_{\rm tot}}.
\end{align}
This is equivalent to \eqref{eq:numerical_probability_bound}.
\end{proof}
